# Supplementary material for: Operating-Envelopes-Aware Decentralized Welfare Maximization for Energy Communities
Source: arXiv:2310.07157 source file (2023-10-11)
Supplement: Supplementary file 1 [file appendix.tex]

\subsection{Proof of Lemma \ref{lem:OptSchedule}}
Recall the community member's surplus-maximization problem under the proposed market mechanism. One can easily see that the objective is both concave and differentiable. From KKT conditions, the optimal consumption of every $i\in \mathcal{N}$ community member is:
$$d^{\ast,\chi}_{ik} = \max\{\underline{d}_{ik}, \min\{f_{ik}(\Gamma^\chi(b_\mathcal{N})),\overline{d}_{ik}\}\}, \quad \forall k \in \mathcal{K}.$$
which can be explicitly written as (in vector form)
\begin{equation}\label{eq:OptdiMember}
       \bm{d}^{\ast,\chi}_i = \begin{cases}
           \bm{d}_i^{\chi^+}(b_\mathcal{N}) &,  b_\mathcal{N} \leq \sigma_1\\
          \bm{d}_i^{\pi^+}&,  b_\mathcal{N} \in [\sigma_1,\sigma_2]\\
           \bm{d}_i^{\chi^z}(b_\mathcal{N})&,  b_\mathcal{N} \in [\sigma_2,\sigma_3]\\
            \bm{d}_i^{\pi^-}&,  b_\mathcal{N} \in [\sigma_3,\sigma_4]\\
            \bm{d}_i^{\chi^-}(b_\mathcal{N})&,  b_\mathcal{N} \geq \sigma_4,
       \end{cases}
   \end{equation}
By definition, the optimal net consumption is
\begin{align*}
z^{\ast,\chi}_i &= \bm{1}^\top \bm{d}^{\ast,\chi}_{i} + r_i - g_i=\bm{1}^\top \bm{d}^{\ast,\chi}_{i}-b_i,\nn
\end{align*}
and the aggregate consumption is $ d_\mathcal{N}^\ast = \sum_{i \in \mathcal{N}} \bm{1}^\top \bm{d}^{\ast,\chi}_i$. Lastly, from (\ref{eq:MonotonicPrices1})-(\ref{eq:MonotonicPrices3}), we, respectively, have 
\begin{align*}
    \sum_{i\in \mathcal{N}} \bm{1}^\top \bm{d}_i^{\chi^+}(b_\mathcal{N}) &= b_\mathcal{N}+\overline{z}_\mathcal{N}\nn\\
    \sum_{i\in \mathcal{N}} \bm{1}^\top \bm{d}_i^{\chi^z}(b_\mathcal{N}) &= b_\mathcal{N}\nn\\
    \sum_{i\in \mathcal{N}} \bm{1}^\top \bm{d}_i^{\chi^-}(b_\mathcal{N}) &= b_\mathcal{N}+\underline{z}_\mathcal{N},\nn
\end{align*}
which yields the aggregate net-consumption
\begin{equation*}
       z^{\ast,\chi}_{\mathcal{N}}(b_\mathcal{N}) = d_\mathcal{N}^\ast - b_\mathcal{N} = \begin{cases}
           \overline{z}_\mathcal{N} &,  b_\mathcal{N} \leq \sigma_1\\
          d_\mathcal{N}^\ast - b_\mathcal{N}&,  b_\mathcal{N} \in [\sigma_1,\sigma_2]\\
           0&,  b_\mathcal{N} \in [\sigma_2,\sigma_3]\\
            d_\mathcal{N}^\ast - b_\mathcal{N}&,  b_\mathcal{N} \in [\sigma_3,\sigma_4]\\
            \underline{z}_\mathcal{N}&,  b_\mathcal{N} \geq \sigma_4.
       \end{cases}
   \end{equation*}
\qed

\subsection{Lemma \ref{lem:BenchmarkSur} and its proof}
\begin{lemma}[Benchmark maximum surplus]\label{lem:BenchmarkSur}
The optimal consumption of standalone customers under the utility's NEM regime abide by the following 4-thresholds,
\begin{align}
 \sigma_1^i &:= \sigma_2^i - \overline{z}_i, \quad \quad \sigma_2^i := \sum_{k \in \mathcal{K}} \max \{ \underline{d}_{ik},\min\{f_{ik}(\pi^+),\overline{d}_{ik}\}\}\label{eq:sigma2}\\
\sigma_3^i &:= \sum_{k\in \mathcal{K}} \max \{\underline{d}_{ik},\min\{f_{ik}(\pi^-),\overline{d}_{ik}\}\},\label{eq:sigma3} \quad \quad
\sigma_4^i := \sigma_3^i - \underline{z}_i.
\end{align}
as 
\begin{equation}\label{eq:OptConsStandalone}
    \bm{d}^{\ast,\pi}_i(b_i) :=\begin{cases}
\bm{d}^{\mu^+}_i(b_i) &, b_i\leq \sigma_1^{i}\\ 
\bm{d}^{\pi^+}_i &, b_i \in [\sigma_1^{i},\sigma_2^{i}]\\ 
\bm{d}^{\mu^o}_i(b_i) &, b_i \in [\sigma_2^{i},\sigma_3^{i}]\\  
\bm{d}^{\pi^-}_i &, b_i \in [\sigma_3^{i},\sigma_4^{i}]\\ 
\bm{d}^{\mu^-}_i(b_i) &, b_i \geq \sigma_4^{i}
\end{cases}
\end{equation}
where the static consumptions $\bm{d}^{\pi^+}_i$ and $\bm{d}^{\pi^-}_i$ and dynamic consumptions $\bm{d}^{\mu^+}_i(b_i),\bm{d}^{\mu^o}_i(b_i),\bm{d}^{\mu^-}_i(b_i)$, for every $k \in \mathcal{K}$, are all given by, 
\begin{equation}\label{eq:d+d-}
    d^x_{ik} := \max \{ \underline{d}_{ik},\min\{f_{ik}(x),\overline{d}_{ik}\}\},
\end{equation}
 and the prices $\mu^+(b_i), \mu^o(b_i), \mu^-(b_i)$ are the solutions of:
 \begin{align}
   \sum_{k \in \mathcal{K}}  \max \{ \underline{d}_{ik},\min\{f_{ik}(\mu_1),\overline{d}_{ik}\}\} &= \overline{z}_i + b_i,\\
   \sum_{k \in \mathcal{K}}  \max \{ \underline{d}_{ik},\min\{f_{ik}(\mu_2),\overline{d}_{ik}\}\} &=  b_i,\\
    \sum_{k \in \mathcal{K}} \max \{ \underline{d}_{ik},\min\{f_{ik}(\mu_3),\overline{d}_{ik}\}\} &= \underline{z}_i + b_i,
 \end{align}
 respectively. By definition, the surplus under optimal consumption is given by:
 \begin{equation}\label{eq:OptSStandalone}
    S^{\ast,\pi}_i(b_i) :=\begin{cases}
U_i(\bm{d}^{\mu^+}_i(b_i)) - \pi^+ \overline{z}_i &, b_i\leq \sigma_1^{i}\\ 
U_i(\bm{d}^{\pi^+}_i) - \pi^+ (\bm{1}^\top \bm{d}^{\pi^+}_i- b_i) &, b_i \in [\sigma_1^{i},\sigma_2^{i}]\\ 
U_i(\bm{d}^{\mu^o}_i(b_i)) &, b_i \in [\sigma_2^{i},\sigma_3^{i}]\\  
U_i(\bm{d}^{\pi^-}_i) - \pi^- (\bm{1}^\top \bm{d}^{\pi^-}_i- b_i) &, b_i \in [\sigma_3^{i},\sigma_4^{i}]\\ 
U_i(\bm{d}^{\mu^-}_i(b_i)) - \pi^- \underline{z}_i &, b_i \geq \sigma_4^{i},
\end{cases}
\end{equation}

\end{lemma}

\subsubsection*{Proof of Lemma \ref{lem:BenchmarkSur}}
For every $i \in \mathcal{N}$, the concave and non-differentiable objective of the grid-aware prosumer optimization above can be divided into the following three convex programs $\mathcal{P}^{\pi,+}_i, \mathcal{P}^{\pi,-}_i$, and $\mathcal{P}^{\pi,o}_i$, which correspond to when $z_i\geq 0, z_i\leq 0$ and $z_i=0$, respectively\footnote{The proof here follows the approach adopted in \cite{Alahmed&Tong:22IEEETSG}.}:
\begin{align} \label{eq:BenchmarkProblem+}
\begin{array}{lll}\mathcal{P}_{i}^{\pi,+}: &  \underset{\bm{d}_i \in \mathbb{R}^K}{\rm minimize}&  \pi^+ (\bm{1}^\top \bm{d}_i - b_i)-U_i(\bm{d}_i)  \\&\text{subject to} & \bm{1}^\top \bm{d}_i - b_i \geq 0 , \\&&
\underline{\bm{d}}_i\preceq \bm{d}_i \preceq \overline{\bm{d}}_i \\&& z_i \leq \overline{z}_i. 
\end{array}   \end{align} 
\begin{align} \label{eq:BenchmarkProblem-}
\begin{array}{lll}\mathcal{P}_{i}^{\pi,-}: &  \underset{\bm{d}_i \in \mathbb{R}^K}{\rm minimize}&  \pi^- (\bm{1}^\top \bm{d}_i - b_i)-U_i(\bm{d}_i)  \\&\text{subject to} & \bm{1}^\top \bm{d}_i - b_i \leq 0 , \\&&
\underline{\bm{d}}_i\preceq \bm{d}_i \preceq \overline{\bm{d}}_i \\&& \underline{z}_i \leq  z_i. 
\end{array}   \end{align} 
\begin{align} \label{eq:BenchmarkProblemo}
\begin{array}{lll}\mathcal{P}_{i}^{\pi,o}: &  \underset{\bm{d}_i \in \mathbb{R}^K}{\rm minimize}&  -U_i(\bm{d}_i)  \\&\text{subject to} & \bm{1}^\top \bm{d}_i - b_i = 0 , \\&&
\underline{\bm{d}}_i\preceq \bm{d}_i \preceq \overline{\bm{d}}_i. 
\end{array}   \end{align} 
Since we assumed that for every $i \in \mathcal{N}$, the OEs ($\overline{z}_i,\underline{z}_i$) satisfy $\overline{z}_i\geq \bm{1}^\top \underline{\bm{d}}_{i} - b_i$ and $\underline{z}_i\leq \bm{1}^\top \overline{\bm{d}}_{i} - b_i$, an optimal solution for all three optimizations above exist. Because the Slater’s condition is satisfied for these optimizations, KKT conditions for optimality are necessary and sufficient. Given $b_i$,  the optimal schedule is the one that achieves the minimum value among $\mathcal{P}_{i}^{\pi,+},\mathcal{P}_{i}^{\pi,-}$ and $\mathcal{P}_{i}^{\pi,o}$. 

\begin{enumerate}[leftmargin=*]
    \item {\em Schedule when $z_i\geq 0$}:\\
    Under $\mathcal{P}_{i}^{\pi,+}$, the Lagrangian $\mathcal{L}^+$ is given by
    \begin{align*}
        \mathcal{L}^+ &= \pi^+ (\sum_{k \in \mathcal{K}} d_{ik} - b_i) - \sum_{k \in \mathcal{K}} U_{ik}(d_{ik})\\& + \sum_{k \in \mathcal{K}} \gamma^+_{ik} (d_{ik}-\overline{d}_{ik})- \sum_{k \in \mathcal{K}}\lambda^+_{ik}(d_{ik}-\underline{d}_{ik})\\& - \kappa^+_i (\sum_{k \in \mathcal{K}} d_{ik} - b_i) + \nu^+_i (\sum_{k \in \mathcal{K}} d_{ik} - b_i - \overline{z}_i),
    \end{align*}
    where $\gamma^+_{ik},\lambda^+_{ik},\kappa^+_{i},\nu^+_i \geq 0$ are Lagrange multipliers for the upper and lower consumption constraints, net-consumption zone constraint, and operating envelop constraint, respectively. Given that the program $\mathcal{P}^o_i$ covers the case when $\kappa^+_i>0$, we can here set $\kappa^+_i=0$. From the KKT conditions we have, for all $k\in \mathcal{K}$,
    \begin{equation*}
        d_{ik}^\ast = f_{ik}(\pi^+ + \gamma^+_{ik} - \lambda^+_{ik} + \nu^+_{ik})
    \end{equation*}
From \cite{Alahmed&Tong:22IEEETSG}, we know that when $\nu^+_{i}=0$ we have $$d^{\ast}_{ik} := \max\{\underline{d}_{ik},\min\{f_{ik}(\pi^+),\overline{d}_{ik}\}\}.$$ When the upper operating envelope is binding, we have $\nu^+_i>0$, and the optimal consumption becomes $$d^{\ast}_{ik} := \max\{\underline{d}_{ik},\min\{f_{ik}(\pi^++\nu^+_i),\overline{d}_{ik}\}\},$$ where the price $\mu_1:=\pi^++\nu^+_i$ is such that the following equality holds:
\begin{equation}\label{eq:Lem1proofNC}
    \sum_{k \in \mathcal{K}} \max\{\underline{d}_{ik},\min\{f_{ik}(\mu_1),\overline{d}_{ik}\}\}-b_i = \overline{z}_i.
\end{equation}
Next, we show that (\ref{eq:Lem1proofNC}) must have a non-negative solution when $b_i \in [\sigma^i_0,\sigma^i_1]$, where $\sigma^i_0 := \bm{1}^\top \underline{\bm{d}}_i -\overline{z}_i$. Let,
\begin{equation}\label{eq:lem1F1}
    F_1(x):= \sum_{k \in \mathcal{K}}\max\{\underline{d}_{ik},\min\{f_{ik}(\mu_1),\overline{d}_{ik}\}\}-b_i - \overline{z}_i.
\end{equation}
which is a continuous and monotonically decreasing function of $b_i$. Since
$$F_1(\pi^+)\geq 0,\quad F_1(\mu_{\mbox{\tiny max}})\leq 0,$$
where $\mu_{\mbox{\tiny max}}$ is such that $$\sum_{k \in \mathcal{K}} \max\{\underline{d}_{ik},\min\{f_{ik}(\mu_{\mbox{\tiny max}}),\overline{d}_{ik}\}\}= \sum_{k \in \mathcal{K}} \underline{d}_{ik},$$ there must exist a $\mu_1 \in [\pi^+,\mu_{\mbox{\tiny max}}]$ such that $F(\mu_1)=0$. The positive solution of (\ref{eq:lem1F1}) also implies 
$${d}^{\mu_1}_{ik}(b_i) \in [\underline{d}_{ik},d_{ik}^{\pi^+}].$$ and from the continuity and monotonicity of $F$ in $b_i$, ${d}^{\mu_1}_{ik}(b_i)$ is also a continuous and monotonically increasing
function of $b_i$.

Hence, in summary:
\begin{align}
&d^{\ast}_{ik}(b_i) =\nonumber\\& \begin{cases}
d^+_{ik}, &\hspace{-.75em} \sum_{k\in K} d^+_{ik} -b_i < \overline{z}_i\\ 
\max\{\underline{d}_{ik},\min\{f_{ik}(\mu^+(b_i)),\overline{d}_{ik}\}\}, &\hspace{-.75em} \sum_{k\in K} d^+_{ik}-b_i \geq \overline{z}_i, \nonumber
\end{cases}
\end{align}
where $d^+_{ik}:=\max\{\underline{d}_{ik},\min\{f_{ik}(\pi^+),\overline{d}_{ik}\}\}$, and $\mu^+(b_i)\geq \pi^+$ is the price that solves (\ref{eq:Lem1proofNC}). From our definition of $\sigma_1$ and $\sigma_2$, we can re-write the optimal consumption above as
$$d^{\ast}_{ik}(b_i) = \begin{cases}
d^+_{ik} &, b_i > \sigma^i_1\\ 
\max\{\underline{d}_{ik},\min\{f_{ik}(\mu^+(b_i)),\overline{d}_{ik}\}\} &, b_i \leq \sigma^i_1.
\end{cases}$$

    \item {\em Schedule when $z_i\leq 0$}:\\
 Under $\mathcal{P}_{i}^{\pi,-}$, the Lagrangian $\mathcal{L}^-$ is given by
  \begin{align*}
        \mathcal{L}^- &= \pi^- (\sum_{k \in \mathcal{K}} d_{ik} - b_i) - \sum_{k \in \mathcal{K}} U_{ik}(d_{ik})\\& + \sum_{k \in \mathcal{K}} \gamma^-_{ik} (d_{ik}-\overline{d}_{ik})- \sum_{k \in \mathcal{K}}\lambda^-_{ik}(d_{ik}-\underline{d}_{ik})\\& + \kappa^-_i (\sum_{k \in \mathcal{K}} d_{ik} - b_i) - \nu^-_i (\sum_{k \in \mathcal{K}} d_{ik} - b_i - \underline{z}_i),
    \end{align*}
    where $\gamma^-_{ik},\lambda^-_{ik},\kappa^-_{i},\nu^-_i \geq 0$ are Lagrange multipliers for the upper and lower consumption constraints, net-consumption zone constraint, and operating envelop constraint, respectively. Following the same steps in the schedule when $z_i\geq 0$, we have, for all $k \in \mathcal{K}$:
    $$d^{\ast}_{ik}(b_i) = \begin{cases}
d^-_{ik}, &\hspace{-0.75em} d^-_{ik}-b_i > \underline{z}_i\\ 
\max\{\underline{d}_{ik},\min\{f_{ik}(\mu^-(b_i)),\overline{d}_{ik}\}\}, &\hspace{-0.75em} d^-_{ik}-b_i \leq \underline{z}_i
\end{cases}$$
where $d^-_{ik}:=\max\{\underline{d}_{ik},\min\{f_{ik}(\pi^-),\overline{d}_{ik}\}\}$, and $\mu^-(b_i) \leq \pi^-$ is the price that solves:
\begin{equation*}
    \sum_{k \in \mathcal{K}} \max\{\underline{d}_{ik},\min\{f_{ik}(\mu_2),\overline{d}_{ik}\}\}-b_i = \underline{z}_i. 
\end{equation*}
From our definition of $\sigma_3^i$ and $\sigma_4^i$, we can re-write the optimal consumption above as
$$d^{\ast}_{ik}(b_i) = \begin{cases}
d^-_{ik} &, b_i < \sigma^i_4\\ 
\max\{\underline{d}_{ik},\min\{f_{ik}(\mu^-),\overline{d}_{ik}\}\} &, b_i \geq \sigma^i_4
\end{cases}$$
Similar to $\mathcal{P}_{i}^{\pi,+}$, we can show that there must exist $\mu^-(b_i) \in [\mu_{\mbox{\tiny min}},\pi^-]$ when $b_i \in [\sigma^i_4,\sigma^i_5]$, where $\sigma^i_5:= \bm{1}^\top \overline{\bm{d}}_i - \underline{z}_i$. Also, the consumption when the export operating envelope $\underline{z}_i$ binds $d^{\mu^-}_{ik}(b_i)$ is continuous and monotonically increasing in $b_i$, and bounded by $d^{\mu^-}_{ik}(b_i) \in [d^{\pi^-}_{ik},\overline{d}_{ik}]$.

    \item {\em Schedule when $z_i= 0$}:\\
    Lastly, the schedule of $\mathcal{P}^o_i$ is exactly the same as in \cite{Alahmed&Tong:22IEEETSG}. Therefore, the optimal consumption, when $b_i \in [\sigma^i_2, \sigma^i_3]$, is 
    \begin{equation*}
        d^{\ast}_{ik}(b_i)= \max\{\underline{d}_{ik},\min\{f_{ik}(\mu^o),\overline{d}_{ik}\}\}\in [\sigma^i_2,\sigma^i_3],
    \end{equation*}
    where $\sigma^i_2, \sigma^i_3$ are as defined in Lemma \ref{lem:BenchmarkSur}, and $\mu^o \in [\pi^-,\pi^+]$ is the solution of:
    \begin{equation*}
    \sum_{k \in \mathcal{K}} \max\{\underline{d}_{ik},\min\{f_{ik}(\mu_3),\overline{d}_{ik}\}\}-b_i = 0. 
\end{equation*}
Combining the three zones, we get the optimal consumption in (\ref{eq:OptConsStandalone}), which given the definition of surplus, yields (\ref{eq:OptSStandalone}). \qed

\end{enumerate}

\subsection{Proof of Theorem \ref{thm:IndRat}}
To prove Theorem \ref{thm:IndRat}, we compare the maximum benchmark surplus ($S_i^{\ast,\pi}$) in Lemma \ref{lem:BenchmarkSur} shown in (\ref{eq:OptSStandalone}) and the maximum community member surplus ($S_i^{\ast,\chi}$) in Lemma \ref{lem:OptSchedule} shown in (\ref{eq:memberOptS}), and show that individual rationality holds, i.e., $\Delta S_i:= S_i^{\ast,\chi} - S_i^{\ast,\pi} \geq 0, \forall i \in \mathcal{N}$. For brevity, we assume a single device case $K=1$, and nonbinding consumption upper and lower limits $\underline{\bm{d}}_i, \overline{\bm{d}}_i, \forall i\in \mathcal{N}$. For notational convenience we define the following:
\begin{align*}
    \overline{y}_i := \left(\overline{z}_i + \frac{\overline{z}_\mathcal{N}-\sum_{i\in \mathcal{N}}\overline{z}_i}{N}\right),
    \underline{y}_i:= \left(\underline{z}_i + \frac{\underline{z}_\mathcal{N}-\sum_{i\in \mathcal{N}}\underline{z}_i}{N}\right).
\end{align*}
hence the fixed reward can be re-written as
\begin{equation*}
     Y^\chi_i(b_\mathcal{N}):= \begin{cases}
(\chi^+(b_\mathcal{N})-\pi^+)\cdot \overline{y}_i, &\hspace{0cm} b_\mathcal{N}\leq \sigma_1 \\ 
(\chi^-(b_\mathcal{N})-\pi^-)\cdot \underline{y}_i, &\hspace{0cm} b_\mathcal{N}\geq \sigma_4\\
0,&\hspace{0cm} \text{otherwise}.
\end{cases}
 \end{equation*}
Given that the piece-wise functions $S_i^{\ast,\pi}$ and $S_i^{\ast,\chi}$ have 5 pieces, their difference $\Delta S_i$ have $5^2$ pieces. The proof is completed if we show that each piece in $\Delta S_i$ is non-negative. In \cite{Alahmed&Tong:23ECjournalarXiv}, we already showed the non-negativity of 9 of the 25 combinations, which are
  \begin{align*}
   1)~b_\mathcal{N}\in [\sigma_1,\sigma_2], b_i \in [\sigma_1^i,\sigma_2^i],2)~ b_\mathcal{N}\in [\sigma_1,\sigma_2], b_i \in [\sigma_2^i,\sigma_3^i]\\
   3)~b_\mathcal{N}\in [\sigma_1,\sigma_2], b_i \in [\sigma_3^i,\sigma_4^i],4)~b_\mathcal{N}\in [\sigma_2,\sigma_3], b_i \in [\sigma_1^i,\sigma_2^i]\\
   5)~b_\mathcal{N}\in [\sigma_2,\sigma_3], b_i \in [\sigma_2^i,\sigma_3^i],6)~b_\mathcal{N}\in [\sigma_2,\sigma_3], b_i \in [\sigma_3^i,\sigma_4^i]\\ 7)~b_\mathcal{N}\in [\sigma_3,\sigma_4], b_i \in [\sigma_1^i,\sigma_2^i],8)~b_\mathcal{N}\in [\sigma_3,\sigma_4], b_i \in [\sigma_2^i,\sigma_3^i]\\
   9)~b_\mathcal{N}\in [\sigma_3,\sigma_4], b_i \in [\sigma_3^i,\sigma_4^i].\hspace{4.35cm}
  \end{align*}
To this end, we prove the non-negativity of the remaining 16 cases using the following inequality for concave and continuously
differentiable function
$$L(x)(y-x)\geq U(y)-U(x)\geq L(y)(y-x),$$
where $x<y, \forall x,y\in \mathbb{R}$.

\begin{description}[align=left,leftmargin = 0pt]
  \item [(Case 1: $b_\mathcal{N} \leq \sigma_1, b_i \leq \sigma_1^i$)] The surplus difference is
  \begin{align*}
   \Delta S_i&=U_i(d^{\chi^+}_i) - \chi^+ ( d^{\chi^+}_i- b_i) +(\chi^+-\pi^+) \overline{y}_i \\&- U_i(d^{\mu^+}_i(b_i))+ \pi^+ \overline{z}_i.
    \end{align*}
    Here we have two sub-cases i) $d^{\chi^+}_i> d^{\mu^+}_i$ and ii) $d^{\chi^+}_i< d^{\mu^+}_i$. Under sub-case (i), we can write
    $$\mu^+ (d^{\chi^+}_i-d^{\mu^+}_i) \geq U_i(d^{\chi^+}_i) - U_i(d^{\mu^+}_i)\geq \chi^+ (d^{\chi^+}_i-d^{\mu^+}_i),$$
    where we used $L_i(d^{\chi^+})= \chi^+$ and $L_i(d^{\mu^+})= \mu^+$. Using the lower bound above, we have
    $$\Delta S_i= (\chi^+-\pi^+)(\overline{y}_i-\overline{z}_i)\geq 0,$$
    where we used $\overline{z}_i= d^{\mu^+}_i - b_i$ when $b_i \leq \sigma_1^i$.\\
    Under sub-case (ii), we have
    $$\chi^+ (d^{\mu^+}_i-d^{\chi^+}_i) \geq  U_i(d^{\mu^+}_i) - U_i(d^{\chi^+}_i)\geq \mu^+ (d^{\mu^+}_i-d^{\chi^+}_i).$$
    By multiplying the inequalities above by $-1$, we get the inequality in sub-case (i) and the proof follows directly.
    
  \item [(Case 2: $b_\mathcal{N} \leq \sigma_1, \sigma_1^i \leq b_i \leq \sigma_2^i$)]  The surplus difference is
  \begin{align*}
   \Delta S_i&=U_i(d^{\chi^+}_i) - \chi^+ ( d^{\chi^+}_i- b_i) +(\chi^+-\pi^+) \overline{y}_i \\&- U_i(d^{\pi^+}_i)+ \pi^+ (d_i^{\pi^+}-b_i).
    \end{align*}
    Since $d^{\chi^+}_i < d^{\pi^+}_i$, we have
    $$\pi^+ (d^{\chi^+}_i-d^{\pi^+}_i) \geq U_i(d^{\chi^+}_i) - U_i(d^{\pi^+}_i)\geq \chi^+ (d^{\chi^+}_i-d^{\pi^+}_i),$$
    and using the lower bound, we get
    $$\Delta S_i= (\chi^+ - \pi^+) (b_i - d^{\pi^+}_i + \overline{y}_i).$$
    We know that $\chi^+ \geq \pi^+$, so we only need to show that $b_i - d^{\pi^+}_i + \overline{y}_i\geq 0$.
    Note that we can reformulate $d^{\pi^+}_i - \overline{z}_i \leq b_i \leq d^{\pi^+}_i$ (from case 2) by adding $\overline{y}_i$ to get
    $$0 \leq \overline{y}_i - \overline{z}_i \leq b_i - d^{\pi^+}_i + \overline{y}_i \leq \overline{y}_i,$$
    which proves that $\Delta S_i= (\chi^+ - \pi^+) (b_i - d^{\pi^+}_i + \overline{y}_i)\geq 0$.
    
  \item [(Case 3: $b_\mathcal{N} \leq \sigma_1, \sigma_2^i \leq b_i \leq \sigma_3^i$)] The surplus difference is
  \begin{align*}
   \Delta S_i&=U_i(d^{\chi^+}_i) - \chi^+ ( d^{\chi^+}_i- b_i) +(\chi^+-\pi^+) \overline{y}_i - U_i(d^{\mu^o}_i).
    \end{align*}
    Since $d^{\chi^+}_i > d^{\mu^o}_i$, we have
  $$\mu^o (d^{\chi^+}_i-d^{\mu^o}_i) \geq U_i(d^{\chi^+}_i) - U_i(d^{\mu^o}_i)\geq \chi^+ (d^{\chi^+}_i-d^{\mu^o}_i),$$
    and using the lower bound, we get
     $$\Delta S_i= \chi^+ (b_i - d^{\mu^o}_i) +(\chi^+ - \pi^+) \overline{y}_i,$$
     but we know that in Case 3, $b_i = d^{\mu^o}_i$, hence 
     $$\Delta S_i= (\chi^+ - \pi^+) \overline{y}_i\geq 0.$$
  \item [(Case 4: $b_\mathcal{N} \leq \sigma_1, \sigma_3^i \leq b_i \leq \sigma_4^i$)]  The surplus difference is
  \begin{align*}
   \Delta S_i&=U_i(d^{\chi^+}_i) - \chi^+ ( d^{\chi^+}_i- b_i) +(\chi^+-\pi^-) \overline{y}_i \\&- U_i(d^{\pi^-}_i)+ \pi^- (d_i^{\pi^-}-b_i).
    \end{align*}
    Since $d^{\chi^+}_i < d^{\pi^-}_i$, we have
    $$\pi^- (d^{\chi^+}_i-d^{\pi^-}_i) \geq U_i(d^{\chi^+}_i) - U_i(d^{\pi^-}_i)\geq \chi^+ (d^{\chi^+}_i-d^{\pi^-}_i),$$
    and using the lower bound, we get
    $$\Delta S_i= (\chi^+ - \pi^-) (b_i - d^{\pi^-}_i + \overline{y}_i).$$
    We know that $\chi^+ \geq \pi^-$, so we only need to show that $b_i - d^{\pi^-}_i + \overline{y}_i\geq 0$.
    Note that we can reformulate $d^{\pi^-}_i \leq b_i \leq d^{\pi^-}_i - \underline{z}_i$ (from case 4) by adding $\overline{y}_i$ to get
    $$0 \leq \overline{y}_i \leq b_i - d^{\pi^-}_i + \overline{y}_i \leq \overline{y}_i - \underline{z}_i,$$
    which proves that $\Delta S_i= (\chi^+ - \pi^-) (b_i - d^{\pi^-}_i + \overline{y}_i)\geq 0$.
  \item [(Case 5: $b_\mathcal{N} \leq \sigma_1, b_i \geq \sigma_4^i$)]  The surplus difference is
  \begin{align*}
   \Delta S_i&=U_i(d^{\chi^+}_i) - \chi^+ ( d^{\chi^+}_i- b_i) +(\chi^+-\pi^+) \overline{y}_i \\&- U_i(d^{\mu^-}_i)+ \pi^- \underline{z}_i.
    \end{align*}
    Since $d^{\chi^+}_i < d^{\mu^-}_i$, we have
    $$\mu^- (d^{\chi^+}_i-d^{\mu^-}_i) \geq U_i(d^{\chi^+}_i) - U_i(d^{\mu^-}_i)\geq \chi^+ (d^{\chi^+}_i-d^{\mu^-}_i),$$
     and using the lower bound and $\underline{z}_i = d^{\mu^-}_i - b_i$, we get
    $$\Delta S_i= (\chi^+ - \mu^-) (b_i - d^{\mu^-}_i) +(\chi^+ - \pi^+) \overline{y}_i\geq 0,$$
    because $b_i \geq d^{\mu^-}_i$.
  \item [(Case 6: $b_\mathcal{N} \geq \sigma_4, b_i \leq \sigma_1^i$)] The surplus difference is
  \begin{align*}
   \Delta S_i&=U_i(d^{\chi^-}_i) - \chi^- ( d^{\chi^-}_i- b_i) +(\chi^--\pi^-) \underline{y}_i \\&- U_i(d^{\mu^+}_i)+ \pi^+ \overline{z}_i.
    \end{align*}
    Since $d^{\chi^-}_i > d^{\mu^+}_i$, we have
     $$\mu^+ (d^{\chi^-}_i-d^{\mu^+}_i) \geq U_i(d^{\chi^-}_i) - U_i(d^{\mu^+}_i)\geq \chi^- (d^{\chi^-}_i-d^{\mu^+}_i),$$
    and using the lower bound and $\overline{z}_i= d^{\mu^+}_i - b_i$, we get
     $$\Delta S_i= (\chi^- - \pi^+) (b_i - d^{\mu^+}_i) +(\chi^- - \pi^-) \underline{y}_i\geq 0$$
     because $\chi^-\leq \pi^- \leq  \pi^+$ and $b_i \leq d^{\mu^+}_i$.
  \item [(Case 7: $b_\mathcal{N} \geq \sigma_4, \sigma_1^i \leq b_i \leq \sigma_2^i$)] The surplus difference is
  \begin{align*}
   \Delta S_i&=U_i(d^{\chi^-}_i) - \chi^- ( d^{\chi^-}_i- b_i) +(\chi^--\pi^-) \underline{y}_i \\&- U_i(d^{\pi^+}_i)+ \pi^+ (d_i^{\pi^+}-b_i).
    \end{align*}
     Since $d^{\chi^-}_i > d^{\pi^+}_i$, we have
    $$\pi^+ (d^{\chi^-}_i-d^{\pi^+}_i) \geq U_i(d^{\chi^-}_i) - U_i(d^{\pi^+}_i)\geq \chi^- (d^{\chi^-}_i-d^{\pi^+}_i),$$
    and using the lower bound, we get
    $$\Delta S_i= (\chi^- - \pi^+) (b_i - d^{\pi^+}_i) +(\chi^- - \pi^-) \underline{y}_i\geq 0$$
    because $\chi^-\leq \pi^- \leq  \pi^+$ and $b_i \leq d^{\pi^+}_i$.
  \item [(Case 8: $b_\mathcal{N} \geq \sigma_4, \sigma_2^i \leq b_i \leq \sigma_3^i$)] The surplus difference is
  \begin{align*}
   \Delta S_i&=U_i(d^{\chi^-}_i) - \chi^- ( d^{\chi^-}_i- b_i) +(\chi^--\pi^-) \underline{y}_i - U_i(d^{\mu^o}_i).
    \end{align*}
     Since $d^{\chi^-}_i > d^{\mu^o}_i$, we have
     $$\mu^o (d^{\chi^-}_i-d^{\mu^o}_i) \geq U_i(d^{\chi^-}_i) - U_i(d^{\mu^o}_i)\geq \chi^- (d^{\chi^-}_i-d^{\mu^o}_i),$$
     and using the lower bound and $d^{\mu^o}_i = b_i$, we get
     $$(\chi^- - \pi^-) \underline{y}_i\geq 0.$$
  \item [(Case 9: $b_\mathcal{N} \geq \sigma_4, \sigma_3^i \leq b_i \leq \sigma_4^i$)] The surplus difference is
  \begin{align*}
   \Delta S_i&=U_i(d^{\chi^-}_i) - \chi^- ( d^{\chi^-}_i- b_i) +(\chi^--\pi^-) \underline{y}_i\\&- U_i(d^{\pi^-}_i)+ \pi^- (d^{\pi^-}_i - b_i).
    \end{align*}
     Since $d^{\chi^-}_i > d^{\pi^-}_i$, we have
     $$\pi^- (d^{\chi^-}_i-d^{\pi^-}_i) \geq U_i(d^{\chi^-}_i) - U_i(d^{\pi^-}_i)\geq \chi^- (d^{\chi^-}_i-d^{\pi^-}_i),$$
     and using the lower bound we get
     $$\Delta S_i=(\chi^- - \pi^-) (b_i - d^{\pi^-}_i+\underline{y}_i).$$
     Note that $\chi^- -\pi^- \leq 0$ and by adding $\overline{y}_i$ to $\sigma_3^i \leq b_i \leq \sigma_4^i$ we get 
     $$\underline{y}_i \leq b_i- d^{\pi^-}_i+\underline{y}_i \leq -\underline{z}_i+\underline{y}_i \leq 0$$
     which proves that $\Delta S_i\geq 0$.
  \item [(Case 10: $b_\mathcal{N} \geq \sigma_4, b_i \geq \sigma_4^i$)] The surplus difference is
  \begin{align*}
   \Delta S_i&=U_i(d^{\chi^-}_i) - \chi^- ( d^{\chi^-}_i- b_i) +(\chi^--\pi^-) \underline{y}_i\\&- U_i(d^{\mu^-}_i)+ \pi^- \underline{z}_i.
    \end{align*}
Here we have two sub-cases i) $d^{\chi^-}_i> d^{\mu^-}_i$ and ii) $d^{\chi^-}_i< d^{\mu^-}_i$. Under sub-case (i), we can write
    $$\mu^- (d^{\chi^-}_i-d^{\mu^-}_i) \geq U_i(d^{\chi^-}_i) - U_i(d^{\mu^-}_i)\geq \chi^- (d^{\chi^-}_i-d^{\mu^-}_i),$$
    Using the lower bound, we get
    $$\Delta S_i= (\chi^--\pi^-)(\underline{y}_i-\underline{z}_i)\geq 0,$$
    where we used $\underline{z}_i= d^{\mu^-}_i - b_i$ when $b_i \geq \sigma_4^i$.\\
    Under sub-case (ii), we have
    $$\chi^- (d^{\mu^-}_i-d^{\chi^-}_i) \geq  U_i(d^{\mu^-}_i) - U_i(d^{\chi^-}_i)\geq \mu^- (d^{\mu^-}_i-d^{\chi^-}_i).$$
    By multiplying the inequalities above by $-1$, we get the inequality in sub-case (i) and the proof follows directly.
    
  \item [(Case 11: $\sigma_1 \leq b_\mathcal{N}\leq \sigma_2, b_i \leq \sigma_1^i$)] The surplus difference is
  \begin{align*}
   \Delta S_i&=U_i(d^{\pi^+}_i) - \pi^+ ( d^{\pi^+}_i- b_i)- U_i(d^{\mu^+}_i)+ \pi^+ \overline{z}_i.
    \end{align*}
    Since $d^{\pi^+}_i > d^{\mu^+}_i$, we have
    $$\mu^+ (d^{\pi^+}_i-d^{\mu^+}_i) \geq  U_i(d^{\pi^+}_i) - U_i(d^{\mu^+}_i)\geq \pi^+ (d^{\pi^+}_i-d^{\mu^+}_i),$$
    and using the lower bound and $\overline{z}_i=d^{\mu^+}_i-b_i$, we get $\Delta S_i\geq 0$.
  \item [(Case 12: $\sigma_1 \leq b_\mathcal{N}\leq \sigma_2, b_i \geq \sigma_4^i$)] The surplus difference is
  \begin{align*}
   \Delta S_i&=U_i(d^{\pi^+}_i) - \pi^+ ( d^{\pi^+}_i- b_i)- U_i(d^{\mu^-}_i)+ \pi^- \underline{z}_i.
    \end{align*}
    Since $d^{\pi^+}_i < d^{\mu^-}_i$, we have
    $$\pi^+ (d^{\pi^+}_i-d^{\mu^-}_i) \leq  U_i(d^{\pi^+}_i) - U_i(d^{\mu^-}_i)\leq \mu^- (d^{\pi^+}_i-d^{\mu^-}_i),$$
    and using the lower bound and $\underline{z}_i=d^{\mu^-}_i-b_i$, we get $\Delta S_i= (\pi^--\pi^+)\underline{z}_i\geq 0$.
  \item [(Case 13: $\sigma_2 \leq b_\mathcal{N}\leq \sigma_3, b_i \leq \sigma_1^i$)] The surplus difference is
  \begin{align*}
   \Delta S_i&=U_i(d^{\chi^z}_i) - \chi^z ( d^{\chi^z}_i- b_i)- U_i(d^{\mu^+}_i)+ \pi^+ \overline{z}_i.
    \end{align*}
    Since $d^{\chi^z}_i > d^{\mu^+}_i$, we have
    $$\mu^+ (d^{\chi^z}_i-d^{\mu^+}_i) \geq  U_i(d^{\chi^z}_i) - U_i(d^{\mu^+}_i)\geq \chi^z (d^{\chi^z}_i-d^{\mu^+}_i),$$
    and using the lower bound and $\overline{z}_i=d^{\mu^+}_i-b_i$, we get $\Delta S_i= (\pi^+ - \chi^z)\overline{z}_i\geq 0$.
  \item [(Case 14: $\sigma_2 \leq b_\mathcal{N}\leq \sigma_3, b_i \geq \sigma_4^i$)] The surplus difference is
  \begin{align*}
   \Delta S_i&=U_i(d^{\chi^z}_i) - \chi^z ( d^{\chi^z}_i- b_i)- U_i(d^{\mu^-}_i)+ \pi^- \underline{z}_i.
    \end{align*}
    Since $d^{\chi^z}_i < d^{\mu^-}_i$, we have
    $$\chi^z (d^{\chi^z}_i-d^{\mu^-}_i) \leq  U_i(d^{\chi^z}_i) - U_i(d^{\mu^-}_i)\leq \mu^- (d^{\chi^z}_i-d^{\mu^-}_i),$$
    and using the lower bound and $\underline{z}_i=d^{\mu^-}_i-b_i$, we get $\Delta S_i= (\pi^--\chi^z)\underline{z}_i\geq 0$.
   \item [(Case 15: $\sigma_3 \leq b_\mathcal{N}\leq \sigma_4, b_i \leq \sigma_1^i$)] The surplus difference is
  \begin{align*}
   \Delta S_i&=U_i(d^{\pi^-}_i) - \pi^- ( d^{\pi^-}_i- b_i)- U_i(d^{\mu^+}_i)+ \pi^+ \overline{z}_i.
    \end{align*}
    Since $d^{\pi^-}_i > d^{\mu^+}_i$, we have
    $$\mu^+ (d^{\pi^-}_i-d^{\mu^+}_i) \geq  U_i(d^{\pi^-}_i) - U_i(d^{\mu^+}_i)\geq \pi^- (d^{\pi^-}_i-d^{\mu^+}_i),$$
    and using the lower bound and $\overline{z}_i=d^{\mu^+}_i-b_i$, we get $\Delta S_i= (\pi^+-\pi^-)\underline{z}_i\geq 0$.
   \item [(Case 16: $\sigma_3 \leq b_\mathcal{N}\leq \sigma_4, b_i \geq \sigma_4^i$)] The surplus difference is
  \begin{align*}
   \Delta S_i&=U_i(d^{\pi^-}_i) - \pi^- ( d^{\pi^-}_i- b_i)- U_i(d^{\mu^-}_i)+ \pi^- \underline{z}_i.
    \end{align*}
    Since $d^{\pi^-}_i < d^{\mu^-}_i$, we have
    $$\pi^- (d^{\pi^-}_i-d^{\mu^-}_i) \leq  U_i(d^{\pi^-}_i) - U_i(d^{\mu^-}_i)\leq \mu^- (d^{\pi^-}_i-d^{\mu^-}_i),$$
    and using the lower bound and $\underline{z}_i=d^{\mu^-}_i-b_i$, we get $\Delta S_i\geq 0$.
\end{description}
\qed

\subsection{Lemma \ref{lem:CentralizedWelfare} and its proof}
\begin{lemma}[Community maximum welfare]\label{lem:CentralizedWelfare}
   The maximum community welfare under centralized resource scheduling is a monotonically increasing function of $b_\mathcal{N}$ and given by
   \begin{align}
       &W^{\ast,\chi}_\mathcal{N}(b_\mathcal{N}) = \nn\\&\begin{cases}
           \sum_{i\in \mathcal{N}} U_i(\bm{d}_i^{\chi^+}(b_\mathcal{N})) - \pi^+ \overline{z}_\mathcal{N},&\hspace{-.75em} b_\mathcal{N} \leq \sigma_1\\
           \sum_{i\in \mathcal{N}} U_i(\bm{d}_i^{\pi^+}) - \pi^+ (\sum_{i\in \mathcal{N}} \bm{1}^\top \bm{d}_i^{\pi^+}- b_\mathcal{N}),&\hspace{-.75em}  b_\mathcal{N} \in [\sigma_1,\sigma_2]\\
           \sum_{i\in \mathcal{N}} U_i(\bm{d}_i^{\chi^z}(b_\mathcal{N})),&\hspace{-.75em}  b_\mathcal{N} \in [\sigma_2,\sigma_3]\\
            \sum_{i\in \mathcal{N}} U_i(\bm{d}_i^{\pi^-}) - \pi^- (\sum_{i\in \mathcal{N}} \bm{1}^\top \bm{d}_i^{\pi^-}- b_\mathcal{N}),&\hspace{-.75em}  b_\mathcal{N} \in [\sigma_3,\sigma_4]\\
            \sum_{i\in \mathcal{N}} U_i(\bm{d}_i^{\chi^-}(b_\mathcal{N})) - \pi^- \underline{z}_\mathcal{N},&\hspace{-.75em}  b_\mathcal{N} \geq \sigma_4,\label{eq:MaxCentralW}
       \end{cases}
   \end{align}
   where the thresholds $\sigma_1-\sigma_4$ are as computed in the {\em market mechanism} and all consumptions are as defined in (\ref{eq:d+d-}).
\end{lemma}

\subsection*{Proof of Lemma \ref{lem:CentralizedWelfare}}

 Recall the community welfare maximization $\mathcal{P}^\chi_\mathcal{N}$
    \begin{align*}
\begin{array}{lll}\mathcal{P}_{\mathcal{N}}^\chi: &  \underset{\{\bm{d}_i\}_{i=1}^N,\{z_i\}_{i=1}^N}{\rm maximize}& W_\mathcal{N}^\pi := \sum_{i\in \mathcal{N}} S_{i}^{\ast,\chi}(z_i,\bm{b}) \\&\text{subject to} & (\ref{eq:Conslimit})-(\ref{eq:Netconsi}), (\ref{eq:Surplusi}), ~ \forall i\in \mathcal{N}\\&& (\ref{eq:NetconsN})-(\ref{eq:Netconslimit}),(\ref{eq:Pcommunity})-(\ref{eq:ProfitNeutrality}).\end{array}  \end{align*} 
which can be reformulated to the following program, given the profit-neutrality condition:
\begin{align*}
\begin{array}{lll}\underset{\{\bm{d}_i\}_{i=1}^N,\{z_i\}_{i=1}^N}{\rm maximize}& W_\mathcal{N}^\chi:=\sum_{i\in \mathcal{N}} U_i(\bm{d}_i) - P^\pi_\mathcal{N}(z_\mathcal{N}) \\\text{subject to} & 
z_\mathcal{N}=\sum_{i\in \mathcal{N}} z_i= \sum_{i\in \mathcal{N}} (\bm{1}^\top \bm{d}_{i} -b_i) \\&\underline{\bm{d}}_i\preceq \bm{d}_i \preceq \overline{\bm{d}}_i,~~ \forall i\in \mathcal{N}\\& \underline{z}_\mathcal{N} \leq  z_\mathcal{N} \leq \overline{z}_\mathcal{N}, \end{array}   \end{align*} 

Given the problem above, and the assumption in (\ref{eq:ZNfeasibility}), the proof directly follows from Lemma \ref{lem:BenchmarkSur}, as it is a generalization of the benchmark customer problem by adding the dimension of community members. Therefore, the optimal aggregate consumption $d^{\ast,\chi}_\mathcal{N}$ and maximum welfare (objective) $W^{\ast,\chi}_\mathcal{N}$ will be functions of $b_\mathcal{N}:= \sum_{i\in \mathcal{N}} b_i$ rather than $b_i$. The optimal consumption of every member under centralized operation is, therefore,
\begin{equation*}
       \bm{d}^{\ast,\chi}_i(b_\mathcal{N}) = \begin{cases}
           \bm{d}_i^{\chi^+}(b_\mathcal{N}) &,  b_\mathcal{N} \leq \sigma_1\\
          \bm{d}_i^{\pi^+}&,  b_\mathcal{N} \in [\sigma_1,\sigma_2]\\
           \bm{d}_i^{\chi^z}(b_\mathcal{N})&,  b_\mathcal{N} \in [\sigma_2,\sigma_3]\\
            \bm{d}_i^{\pi^-}&,  b_\mathcal{N} \in [\sigma_3,\sigma_4]\\
            \bm{d}_i^{\chi^-}(b_\mathcal{N})&,  b_\mathcal{N} \geq \sigma_4,
       \end{cases}
   \end{equation*}
   which yields the aggregate net-consumption
   \begin{equation*}
       z^{\ast,\chi}_{\mathcal{N}}(b_\mathcal{N}) = \begin{cases}
           \overline{z}_\mathcal{N} &,  b_\mathcal{N} \leq \sigma_1\\
          \bm{1}^\top \bm{d}_i^{\pi^+} - b_\mathcal{N}&,  b_\mathcal{N} \in [\sigma_1,\sigma_2]\\
           0&,  b_\mathcal{N} \in [\sigma_2,\sigma_3]\\
            \bm{1}^\top \bm{d}_i^{\pi^-} - b_\mathcal{N}&,  b_\mathcal{N} \in [\sigma_3,\sigma_4]\\
            \underline{z}_\mathcal{N}&,  b_\mathcal{N} \geq \sigma_4.
       \end{cases}
   \end{equation*}
The maximum welfare can be directly computed plugging $d^{\ast,\chi}_\mathcal{N}(b_\mathcal{N})$ and $z^{\ast,\chi}_{\mathcal{N}}(b_\mathcal{N})$ into $W^{\ast,\chi}_\mathcal{N}= \sum_{i\in \mathcal{N}} U_i(\bm{d}^{\ast,\chi}_i(b_\mathcal{N})) - P^{\ast,\pi}_\mathcal{N}(z^{\ast,\chi}_{\mathcal{N}}(b_\mathcal{N}))$, which gives (\ref{eq:MaxCentralW}). \qed

\subsection{Proof of Theorem \ref{thm:MktEff}}
The proof follows directly from Lemma \ref{lem:OptSchedule} and Lemma \ref{lem:CentralizedWelfare}. To show $W_{\mathcal{N}}^{\ast,\chi}(b_{\mathcal{N}}) = \sum_{i \in \mathcal{N}} S^{\ast,\chi}_i(z_i^\ast, b_{\mathcal{N}})$, we note that the LHS is already computed in (\ref{eq:MaxCentralW}), so we only need to compute the RHS. From $\bm{d}^{\ast,\chi}_i,z^{\ast,\chi}_i$ computed in Lemma \ref{lem:CentralizedWelfare}, the surplus of each member is
\begin{align}
&S^{\ast,\chi}_i(z^\ast_i,b_\mathcal{N}) =\nn\\&\begin{cases}   U_i(\bm{d}^{\chi^+}_i) - \chi^+ (\bm{1}^\top \bm{d}^{\chi^+}_i- b_i) +(\chi^+-\pi^+) \overline{z}_\mathcal{N}/N,&\hspace{-.85em} b_\mathcal{N} \leq \sigma_1 \\
U_i(\bm{d}^{\pi^+}_i) - \pi^+ (\bm{1}^\top \bm{d}^{\pi^+}_i- b_i),&\hspace{-1.75em} b_\mathcal{N} \in [\sigma_1, \sigma_2] \\ U_i(\bm{d}^{\chi^z}_i) - \chi^z (\bm{1}^\top \bm{d}^{\chi^z}_i- b_i), &\hspace{-1.75em} b_\mathcal{N} \in[\sigma_2,\sigma_3] \\ U_i(\bm{d}^{\pi^-}_i) - \pi^- (\bm{1}^\top \bm{d}^{\pi^-}_i- b_i),& \hspace{-1.75em}
 b_\mathcal{N} \in[\sigma_3,\sigma_4]\\
 U_i(\bm{d}^{\chi^-}_i) - \chi^- (\bm{1}^\top \bm{d}^{\chi^-}_i- b_i) +(\chi^--\pi^-) \underline{z}_\mathcal{N}/N,& \hspace{-.85em} b_\mathcal{N} \geq \sigma_4.\label{eq:memberOptS}
 \end{cases}
 \end{align}
 From the computation of $\chi^+,\chi^z$ and $\chi^-$, we have that $\sum_{i\in \mathcal{N}}(\bm{1}^\top \bm{d}^{\chi^+}_i- b_i)=\overline{z}_\mathcal{N}, \sum_{i\in \mathcal{N}}(\bm{1}^\top \bm{d}^{\chi^z}_i- b_i)=0$, and $\sum_{i\in \mathcal{N}}(\bm{1}^\top \bm{d}^{\chi^-}_i- b_i)=\underline{z}_\mathcal{N}$ when $b_\mathcal{N}\leq \sigma_1, b_\mathcal{N}\in [\sigma_2, \sigma_3]$, and $b_\mathcal{N}\geq \sigma_4$, respectively. Therefore,
 \begin{align*}
    & \sum_{i\in \mathcal{N}} S^{\ast,\chi}_i(z^\ast_i,b_\mathcal{N})= \\&\begin{cases}
           \sum_{i\in \mathcal{N}} U_i(\bm{d}_i^{\chi^+}(b_\mathcal{N})) - \pi^+ \overline{z}_\mathcal{N},&\hspace{-.75em}  b_\mathcal{N} \leq \sigma_1\\
           \sum_{i\in \mathcal{N}} U_i(\bm{d}_i^{\pi^+}) - \pi^+ (\sum_{i\in \mathcal{N}} \bm{1}^\top \bm{d}_i^{\pi^+}- b_\mathcal{N}),&\hspace{-.75em}  b_\mathcal{N} \in [\sigma_1,\sigma_2]\\
           \sum_{i\in \mathcal{N}} U_i(\bm{d}_i^{\chi^z}(b_\mathcal{N})),&\hspace{-.75em}  b_\mathcal{N} \in [\sigma_2,\sigma_3]\\
            \sum_{i\in \mathcal{N}} U_i(\bm{d}_i^{\pi^-}) - \pi^- (\sum_{i\in \mathcal{N}} \bm{1}^\top \bm{d}_i^{\pi^-}- b_\mathcal{N}),&\hspace{-.75em}  b_\mathcal{N} \in [\sigma_3,\sigma_4]\\
            \sum_{i\in \mathcal{N}} U_i(\bm{d}_i^{\chi^-}(b_\mathcal{N})) - \pi^- \underline{z}_\mathcal{N},&\hspace{-.75em}  b_\mathcal{N} \geq \sigma_4
       \end{cases}\\&= W_{\mathcal{N}}^{\ast,\chi}(b_{\mathcal{N}}).
 \end{align*}
 \qed

\subsection{Proof of Theorem \ref{thm:equity}}
To prove that the market mechanism conforms with the cost-causation principle, we need to show that the six cost-causation axioms are satisfied. 

\begin{enumerate}[leftmargin=*]
\item {\em Individual rationality}: The market mechanism achieves individual rationality as shown in Theorem \ref{thm:IndRat}.
\item {\em Profit-neutrality}: To prove profit neutrality of the market mechanism we need to show that the sum of members' payments is equivalent to the payment of the operator to the utility, i.e., 
$$\Psi_\mathcal{N}^{\pi,\chi}(\bm{z}^{\ast,\chi},b_\mathcal{N}) = \sum_{i\in \mathcal{N}} P^{\chi}_i(z^{\ast,\chi}_i,b_\mathcal{N}) - P^\pi(z^{\ast,\chi}_\mathcal{N})=0,$$
where $\bm{z}^{\ast,\chi}:=(z^{\ast,\chi}_1,\ldots,z^{\ast,\chi}_N)$.
From the market mechanism's payment rule and the community's payment at the revenue meter, we have 
\begin{align*}
    \Psi_\mathcal{N}^{\pi,\chi}(\bm{z}^{\ast,\chi},b_\mathcal{N})&=\Gamma^\chi(b_\mathcal{N}) z^{\ast,\chi}_\mathcal{N} - \sum_{i\in\mathcal{N}} Y^\chi_i(b_\mathcal{N}) - \Gamma^\pi(z^{\ast,\chi}_\mathcal{N}) z^{\ast,\chi}_\mathcal{N},
    \end{align*}
    where
    \begin{align*}
    \Gamma^\chi(b_\mathcal{N}) z^{\ast,\chi}_\mathcal{N}&-\Gamma^\pi(z^{\ast,\chi}_\mathcal{N}) z^{\ast,\chi}_\mathcal{N}=\\&\begin{cases}
           (\chi^+(b_\mathcal{N})-\pi^+)\overline{z}_{\mathcal{N}} &,  b_\mathcal{N} \leq \sigma_1\\
          0&,  b_\mathcal{N} \in [\sigma_1,\sigma_2]\\
           0&,  b_\mathcal{N} \in [\sigma_2,\sigma_3]\\
            0&,  b_\mathcal{N} \in [\sigma_3,\sigma_4]\\
            (\chi^-(b_\mathcal{N})-\pi^-)\underline{z}_{\mathcal{N}}&,  b_\mathcal{N} \geq \sigma_4,
    \end{cases}
    \end{align*}
   and 
\begin{align*}
&\sum_{i\in\mathcal{N}} Y^\chi_i(b_\mathcal{N})=\\& \begin{cases} \sum_{i=1}^N(\chi^+(b_\mathcal{N})-\pi^+) \left(\overline{z}_i + \frac{\overline{z}_\mathcal{N}-\sum_{i\in \mathcal{N}}\overline{z}_i}{N}\right) & ,~ b_\mathcal{N}\leq \sigma_1 \\ 
\sum_{i=1}^N(\chi^-(b_\mathcal{N})-\pi^-) \left(\underline{z}_i + \frac{\underline{z}_\mathcal{N}-\sum_{i\in \mathcal{N}}\underline{z}_i}{N}\right) & ,~ b_\mathcal{N}\geq \sigma_4\\
0&, \text{o.w.}
\end{cases} 
\end{align*}
Calculating the difference gives $\Psi_\mathcal{N}^{\pi,\chi}(\bm{z}^{\ast,\chi},b_\mathcal{N})=0$
\item {\em Equal treatment of equals}: Showing how the market mechanism satisfies this axiom is straightforward, as $z^{\ast,\chi}_i=z^{\ast,\chi}_j$ ($i\neq j$) gives $\tilde{P}^{\chi}_i(z^{\ast,\chi}_i,b_\mathcal{N})=\tilde{P}^{\chi}_j(z^{\ast,\chi}_j,b_\mathcal{N})$. The intuition is that the community price $\Gamma^\chi(b_\mathcal{N})$ is non-discriminatory.
\item {\em Monotonicity}: The fixed-reward-adjusted payments of any two members $i$ and $j$, $i\neq j$, under the market mechanism is given by:
\begin{align*}
    \tilde{P}^{\chi}_i(z_i,b_\mathcal{N})=
\Gamma^{\chi}(b_\mathcal{N})\cdot z_i,~~ \tilde{P}^{\chi}_j(z_j,b_\mathcal{N})=
\Gamma^{\chi}(b_\mathcal{N})\cdot  z_j,
\end{align*}
respectively. One should easily see that, when $|z_i|\geq |z_j|$, and $z_i z_j \geq 0$, it holds that
$$ |\tilde{P}^{\chi}(z_i,b_\mathcal{N})|=
\Gamma^{\chi}(b_\mathcal{N})\cdot |z_i| \geq
\Gamma^{\chi}(b_\mathcal{N})\cdot  |z_j|=|\tilde{P}^{\chi}(z_j,b_\mathcal{N})|.$$
\item {\em Cost causation penalty}: The fixed-reward-adjusted payment clearly obeys the cost-causation penalty axiom, as if $z_i\geq 0, \tilde{P}^{\chi}_i(z_i,b_\mathcal{N})=
\Gamma^{\chi}(b_\mathcal{N})\cdot z_i \geq 0$.
\item {\em Cost mitigation reward}: Cost mitigation reward axiom follows directly from the cost causation reward, as if $z_i\leq 0, \tilde{P}^{\chi}_i(z_i,b_\mathcal{N})=
\Gamma^{\chi}(b_\mathcal{N})\cdot z_i \leq 0$.
\end{enumerate}
From Definition \ref{def:CostCausation}, given that the market mechanism satisfies all six axioms, the market mechanism conforms with the cost-causation principle. \qed
