# Supplementary material for: Operating-Envelopes-Aware Decentralized Welfare Maximization for Energy Communities
Source: arXiv:2310.07157 source file (2023-10-11)
Supplement: Supplementary file 2 [file generalization.tex]

Here, we assume that the benchmark customers may have different OEs, which could be either because the DSO discriminatively assigns OEs within a customer class (e..g, residential), or because the community members do not all belong to a single customer class, i.e., some members may be residential and others may be commercial or agricultural. 

To this end, for every $i \in \mathcal{N}$, the DSO-imposed lower and upper OEs at the benchmark prosumer's revenue meter are denoted by $\underline{z}_i \leq 0$ and $\overline{z}_i \geq 0$, respectively. Therefore, the surplus-maximizing benchmark prosumer solves the following program:
\begin{align} \label{eq:BenchmarkProblemGeneralized}
\hat{\mathcal{P}}_{i}^\pi:   \underset{\bm{d}_i \in \mathbb{R}^K, z_i \in \mathbb{R}}{\rm maximize}~~&  \hat{S}^{\pi}_i(z_i):=U_i(\bm{d}_i) - P^{\pi}(z_i) \nonumber \\\text{subject to}~~ & z_i := \boldsymbol{1}^\top \bm{d}_{i} + r_i -g_i :=\boldsymbol{1}^\top \bm{d}_{i}-b_i , \nonumber \\&
\underline{\bm{d}}_i\preceq \bm{d}_i \preceq \overline{\bm{d}}_i \\& \underline{z}_i \leq  z_i \leq \overline{z}_i, \nonumber
\end{align} 

As a result of this generalization, the payment rule of the proposed grid-aware market mechanism is modified to
\begin{equation}\label{eq:PaymentRuleGeneralized}
\hat{P}^{\chi}(z_i,b_\mathcal{N})=
\underbrace{\Gamma^{\chi}(b_\mathcal{N})\cdot z_i}_\text{volumetric charge} - \underbrace{\hat{Y}^\chi_i(b_\mathcal{N})}_\text{fixed charge},
 \end{equation}
where the pricing rule $\Gamma^{\chi}$ remain as is, but the uniform fixed charge (reward) $Y^\chi(b_\mathcal{N})\geq 0$ becomes non-uniform, as
\begin{equation}\label{eq:fixedrewardGeneralized}
     \hat{Y}^\chi_i(b_\mathcal{N}):= \begin{cases}
(\chi^+(b_\mathcal{N})-\pi^+) \left(\overline{z}_i + \frac{\overline{z}_\mathcal{N}-\sum_{i\in \mathcal{N}}\overline{z}_i}{N}\right), &\hspace{-0.3cm} b_\mathcal{N}\leq \sigma_1 \\ 
(\chi^-(b_\mathcal{N})-\pi^-) \left(\underline{z}_i + \frac{\underline{z}_\mathcal{N}-\sum_{i\in \mathcal{N}}\underline{z}_i}{N}\right), &\hspace{-0.3cm} b_\mathcal{N}\geq \sigma_4\\
0,&\hspace{-0.3cm} \text{otherwise}.
\end{cases}
 \end{equation}
Note that the fixed reward each customer gets $\hat{Y}_i^\chi(b_\mathcal{N})$ is proportional with their benchmark's OEs $\underline{z}_i,\overline{z}_i$. The intuition of this is that the operator needs to reward customers with better (less restrictive) OEs more to ensure that they have enough incentive to join the community, which leads to the generalized version of the individual rationality theorem.

\begin{theorem*}[Individual rationality under non-uniform OEs]\label{thm:IndRatGeneralized}
    Under the proposed market mechanism, and assuming that $\sum_{i\in \mathcal{N}} \overline{z}_i \leq \overline{z}_\mathcal{N}$ and $\sum_{i\in \mathcal{N}} \underline{z}_i \geq \underline{z}_\mathcal{N}$, every $i \in \mathcal{N}$ member achieves a surplus no less than its benchmark, i.e.,
\begin{equation}\label{eq:Sopt2Benchmark_moel2Generalized}
    S^{\ast,\chi}_i(z^{\ast,\chi}_i,b_\mathcal{N}) \geq S^{\ast,\pi}_i(b_i).
\end{equation}
\end{theorem*}
\noindent {\em Proof:}
The proof of the generalized individual rationality theorem under non-uniform OEs follows directly form the proof of Theorem \ref{thm:IndRat}.
