# Supplementary material for: Operating-Envelopes-Aware Decentralized Welfare Maximization for Energy Communities
Source: arXiv:2310.07157 source file (2023-10-11)
Supplement: Supplementary file 4 [file Eff.tex]

The proof follows directly from Lemma \ref{lem:OptSchedule} and Lemma \ref{lem:CentralizedWelfare}. To show $W_{\mathcal{N}}^{\ast,\chi}(b_{\mathcal{N}}) = \sum_{i \in \mathcal{N}} S^{\ast,\chi}_i(z_i^\ast, b_{\mathcal{N}})$, we note that the LHS is already computed in (\ref{eq:MaxCentralW}), so we only need to compute the RHS. From $\bm{d}^{\ast,\chi}_i,z^{\ast,\chi}_i$ computed in Lemma \ref{lem:CentralizedWelfare}, the surplus of each member is
\begin{align}
&S^{\ast,\chi}_i(z^\ast_i,b_\mathcal{N}) =\nn\\&\begin{cases}   U_i(\bm{d}^{\chi^+}_i) - \chi^+ (\bm{1}^\top \bm{d}^{\chi^+}_i- b_i) +(\chi^+-\pi^+) \overline{z}_\mathcal{N}/N,&\hspace{-.85em} b_\mathcal{N} \leq \sigma_1 \\
U_i(\bm{d}^{\pi^+}_i) - \pi^+ (\bm{1}^\top \bm{d}^{\pi^+}_i- b_i),&\hspace{-1.75em} b_\mathcal{N} \in [\sigma_1, \sigma_2] \\ U_i(\bm{d}^{\chi^z}_i) - \chi^z (\bm{1}^\top \bm{d}^{\chi^z}_i- b_i), &\hspace{-1.75em} b_\mathcal{N} \in[\sigma_2,\sigma_3] \\ U_i(\bm{d}^{\pi^-}_i) - \pi^- (\bm{1}^\top \bm{d}^{\pi^-}_i- b_i),& \hspace{-1.75em}
 b_\mathcal{N} \in[\sigma_3,\sigma_4]\\
 U_i(\bm{d}^{\chi^-}_i) - \chi^- (\bm{1}^\top \bm{d}^{\chi^-}_i- b_i) +(\chi^--\pi^-) \underline{z}_\mathcal{N}/N,& \hspace{-.85em} b_\mathcal{N} \geq \sigma_4.\label{eq:memberOptS}
 \end{cases}
 \end{align}
 From the computation of $\chi^+,\chi^z$ and $\chi^-$, we have that $\sum_{i\in \mathcal{N}}(\bm{1}^\top \bm{d}^{\chi^+}_i- b_i)=\overline{z}_\mathcal{N}, \sum_{i\in \mathcal{N}}(\bm{1}^\top \bm{d}^{\chi^z}_i- b_i)=0$, and $\sum_{i\in \mathcal{N}}(\bm{1}^\top \bm{d}^{\chi^-}_i- b_i)=\underline{z}_\mathcal{N}$ when $b_\mathcal{N}\leq \sigma_1, b_\mathcal{N}\in [\sigma_2, \sigma_3]$, and $b_\mathcal{N}\geq \sigma_4$, respectively. Therefore,
 \begin{align*}
    & \sum_{i\in \mathcal{N}} S^{\ast,\chi}_i(z^\ast_i,b_\mathcal{N})= \\&\begin{cases}
           \sum_{i\in \mathcal{N}} U_i(\bm{d}_i^{\chi^+}(b_\mathcal{N})) - \pi^+ \overline{z}_\mathcal{N},&\hspace{-.75em}  b_\mathcal{N} \leq \sigma_1\\
           \sum_{i\in \mathcal{N}} U_i(\bm{d}_i^{\pi^+}) - \pi^+ (\sum_{i\in \mathcal{N}} \bm{1}^\top \bm{d}_i^{\pi^+}- b_\mathcal{N}),&\hspace{-.75em}  b_\mathcal{N} \in [\sigma_1,\sigma_2]\\
           \sum_{i\in \mathcal{N}} U_i(\bm{d}_i^{\chi^z}(b_\mathcal{N})),&\hspace{-.75em}  b_\mathcal{N} \in [\sigma_2,\sigma_3]\\
            \sum_{i\in \mathcal{N}} U_i(\bm{d}_i^{\pi^-}) - \pi^- (\sum_{i\in \mathcal{N}} \bm{1}^\top \bm{d}_i^{\pi^-}- b_\mathcal{N}),&\hspace{-.75em}  b_\mathcal{N} \in [\sigma_3,\sigma_4]\\
            \sum_{i\in \mathcal{N}} U_i(\bm{d}_i^{\chi^-}(b_\mathcal{N})) - \pi^- \underline{z}_\mathcal{N},&\hspace{-.75em}  b_\mathcal{N} \geq \sigma_4
       \end{cases}\\&= W_{\mathcal{N}}^{\ast,\chi}(b_{\mathcal{N}}).
 \end{align*}
 \qed
