# Supplementary material for: Operating-Envelopes-Aware Decentralized Welfare Maximization for Energy Communities
Source: arXiv:2310.07157 source file (2023-10-11)
Supplement: Supplementary file 5 [file Equity.tex]

To prove that the market mechanism conforms with the cost-causation principle, we need to show that the six cost-causation axioms are satisfied. 

\begin{enumerate}[leftmargin=*]
\item {\em Individual rationality}: The market mechanism achieves individual rationality as shown in Theorem \ref{thm:IndRat}.
\item {\em Profit-neutrality}: To prove profit neutrality of the market mechanism we need to show that the sum of members' payments is equivalent to the payment of the operator to the utility, i.e., 
$$\Psi_\mathcal{N}^{\pi,\chi}(\bm{z}^{\ast,\chi},b_\mathcal{N}) = \sum_{i\in \mathcal{N}} P^{\chi}_i(z^{\ast,\chi}_i,b_\mathcal{N}) - P^\pi(z^{\ast,\chi}_\mathcal{N})=0,$$
where $\bm{z}^{\ast,\chi}:=(z^{\ast,\chi}_1,\ldots,z^{\ast,\chi}_N)$.
From the market mechanism's payment rule and the community's payment at the revenue meter, we have 
\begin{align*}
    \Psi_\mathcal{N}^{\pi,\chi}(\bm{z}^{\ast,\chi},b_\mathcal{N})&=\Gamma^\chi(b_\mathcal{N}) z^{\ast,\chi}_\mathcal{N} - \sum_{i\in\mathcal{N}} Y^\chi_i(b_\mathcal{N}) - \Gamma^\pi(z^{\ast,\chi}_\mathcal{N}) z^{\ast,\chi}_\mathcal{N},
    \end{align*}
    where
    \begin{align*}
    \Gamma^\chi(b_\mathcal{N}) z^{\ast,\chi}_\mathcal{N}&-\Gamma^\pi(z^{\ast,\chi}_\mathcal{N}) z^{\ast,\chi}_\mathcal{N}=\\&\begin{cases}
           (\chi^+(b_\mathcal{N})-\pi^+)\overline{z}_{\mathcal{N}} &,  b_\mathcal{N} \leq \sigma_1\\
          0&,  b_\mathcal{N} \in [\sigma_1,\sigma_2]\\
           0&,  b_\mathcal{N} \in [\sigma_2,\sigma_3]\\
            0&,  b_\mathcal{N} \in [\sigma_3,\sigma_4]\\
            (\chi^-(b_\mathcal{N})-\pi^-)\underline{z}_{\mathcal{N}}&,  b_\mathcal{N} \geq \sigma_4,
    \end{cases}
    \end{align*}
   and 
\begin{align*}
&\sum_{i\in\mathcal{N}} Y^\chi_i(b_\mathcal{N})=\\& \begin{cases} \sum_{i=1}^N(\chi^+(b_\mathcal{N})-\pi^+) \left(\overline{z}_i + \frac{\overline{z}_\mathcal{N}-\sum_{i\in \mathcal{N}}\overline{z}_i}{N}\right) & ,~ b_\mathcal{N}\leq \sigma_1 \\ 
\sum_{i=1}^N(\chi^-(b_\mathcal{N})-\pi^-) \left(\underline{z}_i + \frac{\underline{z}_\mathcal{N}-\sum_{i\in \mathcal{N}}\underline{z}_i}{N}\right) & ,~ b_\mathcal{N}\geq \sigma_4\\
0&, \text{o.w.}
\end{cases} 
\end{align*}
Calculating the difference gives $\Psi_\mathcal{N}^{\pi,\chi}(\bm{z}^{\ast,\chi},b_\mathcal{N})=0$
\item {\em Equal treatment of equals}: Showing how the market mechanism satisfies this axiom is straightforward, as $z^{\ast,\chi}_i=z^{\ast,\chi}_j$ ($i\neq j$) gives $\tilde{P}^{\chi}_i(z^{\ast,\chi}_i,b_\mathcal{N})=\tilde{P}^{\chi}_j(z^{\ast,\chi}_j,b_\mathcal{N})$. The intuition is that the community price $\Gamma^\chi(b_\mathcal{N})$ is non-discriminatory.
\item {\em Monotonicity}: The fixed-reward-adjusted payments of any two members $i$ and $j$, $i\neq j$, under the market mechanism is given by:
\begin{align*}
    \tilde{P}^{\chi}_i(z_i,b_\mathcal{N})=
\Gamma^{\chi}(b_\mathcal{N})\cdot z_i,~~ \tilde{P}^{\chi}_j(z_j,b_\mathcal{N})=
\Gamma^{\chi}(b_\mathcal{N})\cdot  z_j,
\end{align*}
respectively. One should easily see that, when $|z_i|\geq |z_j|$, and $z_i z_j \geq 0$, it holds that
$$ |\tilde{P}^{\chi}(z_i,b_\mathcal{N})|=
\Gamma^{\chi}(b_\mathcal{N})\cdot |z_i| \geq
\Gamma^{\chi}(b_\mathcal{N})\cdot  |z_j|=|\tilde{P}^{\chi}(z_j,b_\mathcal{N})|.$$
\item {\em Cost causation penalty}: The fixed-reward-adjusted payment clearly obeys the cost-causation penalty axiom, as if $z_i\geq 0, \tilde{P}^{\chi}_i(z_i,b_\mathcal{N})=
\Gamma^{\chi}(b_\mathcal{N})\cdot z_i \geq 0$.
\item {\em Cost mitigation reward}: Cost mitigation reward axiom follows directly from the cost causation reward, as if $z_i\leq 0, \tilde{P}^{\chi}_i(z_i,b_\mathcal{N})=
\Gamma^{\chi}(b_\mathcal{N})\cdot z_i \leq 0$.
\end{enumerate}
From Definition \ref{def:CostCausation}, given that the market mechanism satisfies all six axioms, the market mechanism conforms with the cost-causation principle. \qed
