# Supplementary material for: Operating-Envelopes-Aware Decentralized Welfare Maximization for Energy Communities
Source: arXiv:2310.07157 source file (2023-10-11)
Supplement: Supplementary file 6 [file IndRat.tex]

To prove Theorem \ref{thm:IndRat}, we compare the maximum benchmark surplus ($S_i^{\ast,\pi}$) in Lemma \ref{lem:BenchmarkSur} shown in (\ref{eq:OptSStandalone}) and the maximum community member surplus ($S_i^{\ast,\chi}$) in Lemma \ref{lem:OptSchedule} shown in (\ref{eq:memberOptS}), and show that individual rationality holds, i.e., $\Delta S_i:= S_i^{\ast,\chi} - S_i^{\ast,\pi} \geq 0, \forall i \in \mathcal{N}$. For brevity, we assume a single device case $K=1$, and nonbinding consumption upper and lower limits $\underline{\bm{d}}_i, \overline{\bm{d}}_i, \forall i\in \mathcal{N}$. For notational convenience we define the following:
\begin{align*}
    \overline{y}_i := \left(\overline{z}_i + \frac{\overline{z}_\mathcal{N}-\sum_{i\in \mathcal{N}}\overline{z}_i}{N}\right),
    \underline{y}_i:= \left(\underline{z}_i + \frac{\underline{z}_\mathcal{N}-\sum_{i\in \mathcal{N}}\underline{z}_i}{N}\right).
\end{align*}
hence the fixed reward can be re-written as
\begin{equation*}
     Y^\chi_i(b_\mathcal{N}):= \begin{cases}
(\chi^+(b_\mathcal{N})-\pi^+)\cdot \overline{y}_i, &\hspace{0cm} b_\mathcal{N}\leq \sigma_1 \\ 
(\chi^-(b_\mathcal{N})-\pi^-)\cdot \underline{y}_i, &\hspace{0cm} b_\mathcal{N}\geq \sigma_4\\
0,&\hspace{0cm} \text{otherwise}.
\end{cases}
 \end{equation*}
Given that the piece-wise functions $S_i^{\ast,\pi}$ and $S_i^{\ast,\chi}$ have 5 pieces, their difference $\Delta S_i$ have $5^2$ pieces. The proof is completed if we show that each piece in $\Delta S_i$ is non-negative. In \cite{Alahmed&Tong:23ECjournalarXiv}, we already showed the non-negativity of 9 of the 25 combinations, which are
  \begin{align*}
   1)~b_\mathcal{N}\in [\sigma_1,\sigma_2], b_i \in [\sigma_1^i,\sigma_2^i],2)~ b_\mathcal{N}\in [\sigma_1,\sigma_2], b_i \in [\sigma_2^i,\sigma_3^i]\\
   3)~b_\mathcal{N}\in [\sigma_1,\sigma_2], b_i \in [\sigma_3^i,\sigma_4^i],4)~b_\mathcal{N}\in [\sigma_2,\sigma_3], b_i \in [\sigma_1^i,\sigma_2^i]\\
   5)~b_\mathcal{N}\in [\sigma_2,\sigma_3], b_i \in [\sigma_2^i,\sigma_3^i],6)~b_\mathcal{N}\in [\sigma_2,\sigma_3], b_i \in [\sigma_3^i,\sigma_4^i]\\ 7)~b_\mathcal{N}\in [\sigma_3,\sigma_4], b_i \in [\sigma_1^i,\sigma_2^i],8)~b_\mathcal{N}\in [\sigma_3,\sigma_4], b_i \in [\sigma_2^i,\sigma_3^i]\\
   9)~b_\mathcal{N}\in [\sigma_3,\sigma_4], b_i \in [\sigma_3^i,\sigma_4^i].\hspace{4.35cm}
  \end{align*}
To this end, we prove the non-negativity of the remaining 16 cases using the following inequality for concave and continuously
differentiable function
$$L(x)(y-x)\geq U(y)-U(x)\geq L(y)(y-x),$$
where $x<y, \forall x,y\in \mathbb{R}$.

\begin{description}[align=left,leftmargin = 0pt]
  \item [(Case 1: $b_\mathcal{N} \leq \sigma_1, b_i \leq \sigma_1^i$)] The surplus difference is
  \begin{align*}
   \Delta S_i&=U_i(d^{\chi^+}_i) - \chi^+ ( d^{\chi^+}_i- b_i) +(\chi^+-\pi^+) \overline{y}_i \\&- U_i(d^{\mu^+}_i(b_i))+ \pi^+ \overline{z}_i.
    \end{align*}
    Here we have two sub-cases i) $d^{\chi^+}_i> d^{\mu^+}_i$ and ii) $d^{\chi^+}_i< d^{\mu^+}_i$. Under sub-case (i), we can write
    $$\mu^+ (d^{\chi^+}_i-d^{\mu^+}_i) \geq U_i(d^{\chi^+}_i) - U_i(d^{\mu^+}_i)\geq \chi^+ (d^{\chi^+}_i-d^{\mu^+}_i),$$
    where we used $L_i(d^{\chi^+})= \chi^+$ and $L_i(d^{\mu^+})= \mu^+$. Using the lower bound above, we have
    $$\Delta S_i= (\chi^+-\pi^+)(\overline{y}_i-\overline{z}_i)\geq 0,$$
    where we used $\overline{z}_i= d^{\mu^+}_i - b_i$ when $b_i \leq \sigma_1^i$.\\
    Under sub-case (ii), we have
    $$\chi^+ (d^{\mu^+}_i-d^{\chi^+}_i) \geq  U_i(d^{\mu^+}_i) - U_i(d^{\chi^+}_i)\geq \mu^+ (d^{\mu^+}_i-d^{\chi^+}_i).$$
    By multiplying the inequalities above by $-1$, we get the inequality in sub-case (i) and the proof follows directly.
    
  \item [(Case 2: $b_\mathcal{N} \leq \sigma_1, \sigma_1^i \leq b_i \leq \sigma_2^i$)]  The surplus difference is
  \begin{align*}
   \Delta S_i&=U_i(d^{\chi^+}_i) - \chi^+ ( d^{\chi^+}_i- b_i) +(\chi^+-\pi^+) \overline{y}_i \\&- U_i(d^{\pi^+}_i)+ \pi^+ (d_i^{\pi^+}-b_i).
    \end{align*}
    Since $d^{\chi^+}_i < d^{\pi^+}_i$, we have
    $$\pi^+ (d^{\chi^+}_i-d^{\pi^+}_i) \geq U_i(d^{\chi^+}_i) - U_i(d^{\pi^+}_i)\geq \chi^+ (d^{\chi^+}_i-d^{\pi^+}_i),$$
    and using the lower bound, we get
    $$\Delta S_i= (\chi^+ - \pi^+) (b_i - d^{\pi^+}_i + \overline{y}_i).$$
    We know that $\chi^+ \geq \pi^+$, so we only need to show that $b_i - d^{\pi^+}_i + \overline{y}_i\geq 0$.
    Note that we can reformulate $d^{\pi^+}_i - \overline{z}_i \leq b_i \leq d^{\pi^+}_i$ (from case 2) by adding $\overline{y}_i$ to get
    $$0 \leq \overline{y}_i - \overline{z}_i \leq b_i - d^{\pi^+}_i + \overline{y}_i \leq \overline{y}_i,$$
    which proves that $\Delta S_i= (\chi^+ - \pi^+) (b_i - d^{\pi^+}_i + \overline{y}_i)\geq 0$.
    
  \item [(Case 3: $b_\mathcal{N} \leq \sigma_1, \sigma_2^i \leq b_i \leq \sigma_3^i$)] The surplus difference is
  \begin{align*}
   \Delta S_i&=U_i(d^{\chi^+}_i) - \chi^+ ( d^{\chi^+}_i- b_i) +(\chi^+-\pi^+) \overline{y}_i - U_i(d^{\mu^o}_i).
    \end{align*}
    Since $d^{\chi^+}_i > d^{\mu^o}_i$, we have
  $$\mu^o (d^{\chi^+}_i-d^{\mu^o}_i) \geq U_i(d^{\chi^+}_i) - U_i(d^{\mu^o}_i)\geq \chi^+ (d^{\chi^+}_i-d^{\mu^o}_i),$$
    and using the lower bound, we get
     $$\Delta S_i= \chi^+ (b_i - d^{\mu^o}_i) +(\chi^+ - \pi^+) \overline{y}_i,$$
     but we know that in Case 3, $b_i = d^{\mu^o}_i$, hence 
     $$\Delta S_i= (\chi^+ - \pi^+) \overline{y}_i\geq 0.$$
  \item [(Case 4: $b_\mathcal{N} \leq \sigma_1, \sigma_3^i \leq b_i \leq \sigma_4^i$)]  The surplus difference is
  \begin{align*}
   \Delta S_i&=U_i(d^{\chi^+}_i) - \chi^+ ( d^{\chi^+}_i- b_i) +(\chi^+-\pi^-) \overline{y}_i \\&- U_i(d^{\pi^-}_i)+ \pi^- (d_i^{\pi^-}-b_i).
    \end{align*}
    Since $d^{\chi^+}_i < d^{\pi^-}_i$, we have
    $$\pi^- (d^{\chi^+}_i-d^{\pi^-}_i) \geq U_i(d^{\chi^+}_i) - U_i(d^{\pi^-}_i)\geq \chi^+ (d^{\chi^+}_i-d^{\pi^-}_i),$$
    and using the lower bound, we get
    $$\Delta S_i= (\chi^+ - \pi^-) (b_i - d^{\pi^-}_i + \overline{y}_i).$$
    We know that $\chi^+ \geq \pi^-$, so we only need to show that $b_i - d^{\pi^-}_i + \overline{y}_i\geq 0$.
    Note that we can reformulate $d^{\pi^-}_i \leq b_i \leq d^{\pi^-}_i - \underline{z}_i$ (from case 4) by adding $\overline{y}_i$ to get
    $$0 \leq \overline{y}_i \leq b_i - d^{\pi^-}_i + \overline{y}_i \leq \overline{y}_i - \underline{z}_i,$$
    which proves that $\Delta S_i= (\chi^+ - \pi^-) (b_i - d^{\pi^-}_i + \overline{y}_i)\geq 0$.
  \item [(Case 5: $b_\mathcal{N} \leq \sigma_1, b_i \geq \sigma_4^i$)]  The surplus difference is
  \begin{align*}
   \Delta S_i&=U_i(d^{\chi^+}_i) - \chi^+ ( d^{\chi^+}_i- b_i) +(\chi^+-\pi^+) \overline{y}_i \\&- U_i(d^{\mu^-}_i)+ \pi^- \underline{z}_i.
    \end{align*}
    Since $d^{\chi^+}_i < d^{\mu^-}_i$, we have
    $$\mu^- (d^{\chi^+}_i-d^{\mu^-}_i) \geq U_i(d^{\chi^+}_i) - U_i(d^{\mu^-}_i)\geq \chi^+ (d^{\chi^+}_i-d^{\mu^-}_i),$$
     and using the lower bound and $\underline{z}_i = d^{\mu^-}_i - b_i$, we get
    $$\Delta S_i= (\chi^+ - \mu^-) (b_i - d^{\mu^-}_i) +(\chi^+ - \pi^+) \overline{y}_i\geq 0,$$
    because $b_i \geq d^{\mu^-}_i$.
  \item [(Case 6: $b_\mathcal{N} \geq \sigma_4, b_i \leq \sigma_1^i$)] The surplus difference is
  \begin{align*}
   \Delta S_i&=U_i(d^{\chi^-}_i) - \chi^- ( d^{\chi^-}_i- b_i) +(\chi^--\pi^-) \underline{y}_i \\&- U_i(d^{\mu^+}_i)+ \pi^+ \overline{z}_i.
    \end{align*}
    Since $d^{\chi^-}_i > d^{\mu^+}_i$, we have
     $$\mu^+ (d^{\chi^-}_i-d^{\mu^+}_i) \geq U_i(d^{\chi^-}_i) - U_i(d^{\mu^+}_i)\geq \chi^- (d^{\chi^-}_i-d^{\mu^+}_i),$$
    and using the lower bound and $\overline{z}_i= d^{\mu^+}_i - b_i$, we get
     $$\Delta S_i= (\chi^- - \pi^+) (b_i - d^{\mu^+}_i) +(\chi^- - \pi^-) \underline{y}_i\geq 0$$
     because $\chi^-\leq \pi^- \leq  \pi^+$ and $b_i \leq d^{\mu^+}_i$.
  \item [(Case 7: $b_\mathcal{N} \geq \sigma_4, \sigma_1^i \leq b_i \leq \sigma_2^i$)] The surplus difference is
  \begin{align*}
   \Delta S_i&=U_i(d^{\chi^-}_i) - \chi^- ( d^{\chi^-}_i- b_i) +(\chi^--\pi^-) \underline{y}_i \\&- U_i(d^{\pi^+}_i)+ \pi^+ (d_i^{\pi^+}-b_i).
    \end{align*}
     Since $d^{\chi^-}_i > d^{\pi^+}_i$, we have
    $$\pi^+ (d^{\chi^-}_i-d^{\pi^+}_i) \geq U_i(d^{\chi^-}_i) - U_i(d^{\pi^+}_i)\geq \chi^- (d^{\chi^-}_i-d^{\pi^+}_i),$$
    and using the lower bound, we get
    $$\Delta S_i= (\chi^- - \pi^+) (b_i - d^{\pi^+}_i) +(\chi^- - \pi^-) \underline{y}_i\geq 0$$
    because $\chi^-\leq \pi^- \leq  \pi^+$ and $b_i \leq d^{\pi^+}_i$.
  \item [(Case 8: $b_\mathcal{N} \geq \sigma_4, \sigma_2^i \leq b_i \leq \sigma_3^i$)] The surplus difference is
  \begin{align*}
   \Delta S_i&=U_i(d^{\chi^-}_i) - \chi^- ( d^{\chi^-}_i- b_i) +(\chi^--\pi^-) \underline{y}_i - U_i(d^{\mu^o}_i).
    \end{align*}
     Since $d^{\chi^-}_i > d^{\mu^o}_i$, we have
     $$\mu^o (d^{\chi^-}_i-d^{\mu^o}_i) \geq U_i(d^{\chi^-}_i) - U_i(d^{\mu^o}_i)\geq \chi^- (d^{\chi^-}_i-d^{\mu^o}_i),$$
     and using the lower bound and $d^{\mu^o}_i = b_i$, we get
     $$(\chi^- - \pi^-) \underline{y}_i\geq 0.$$
  \item [(Case 9: $b_\mathcal{N} \geq \sigma_4, \sigma_3^i \leq b_i \leq \sigma_4^i$)] The surplus difference is
  \begin{align*}
   \Delta S_i&=U_i(d^{\chi^-}_i) - \chi^- ( d^{\chi^-}_i- b_i) +(\chi^--\pi^-) \underline{y}_i\\&- U_i(d^{\pi^-}_i)+ \pi^- (d^{\pi^-}_i - b_i).
    \end{align*}
     Since $d^{\chi^-}_i > d^{\pi^-}_i$, we have
     $$\pi^- (d^{\chi^-}_i-d^{\pi^-}_i) \geq U_i(d^{\chi^-}_i) - U_i(d^{\pi^-}_i)\geq \chi^- (d^{\chi^-}_i-d^{\pi^-}_i),$$
     and using the lower bound we get
     $$\Delta S_i=(\chi^- - \pi^-) (b_i - d^{\pi^-}_i+\underline{y}_i).$$
     Note that $\chi^- -\pi^- \leq 0$ and by adding $\overline{y}_i$ to $\sigma_3^i \leq b_i \leq \sigma_4^i$ we get 
     $$\underline{y}_i \leq b_i- d^{\pi^-}_i+\underline{y}_i \leq -\underline{z}_i+\underline{y}_i \leq 0$$
     which proves that $\Delta S_i\geq 0$.
  \item [(Case 10: $b_\mathcal{N} \geq \sigma_4, b_i \geq \sigma_4^i$)] The surplus difference is
  \begin{align*}
   \Delta S_i&=U_i(d^{\chi^-}_i) - \chi^- ( d^{\chi^-}_i- b_i) +(\chi^--\pi^-) \underline{y}_i\\&- U_i(d^{\mu^-}_i)+ \pi^- \underline{z}_i.
    \end{align*}
Here we have two sub-cases i) $d^{\chi^-}_i> d^{\mu^-}_i$ and ii) $d^{\chi^-}_i< d^{\mu^-}_i$. Under sub-case (i), we can write
    $$\mu^- (d^{\chi^-}_i-d^{\mu^-}_i) \geq U_i(d^{\chi^-}_i) - U_i(d^{\mu^-}_i)\geq \chi^- (d^{\chi^-}_i-d^{\mu^-}_i),$$
    Using the lower bound, we get
    $$\Delta S_i= (\chi^--\pi^-)(\underline{y}_i-\underline{z}_i)\geq 0,$$
    where we used $\underline{z}_i= d^{\mu^-}_i - b_i$ when $b_i \geq \sigma_4^i$.\\
    Under sub-case (ii), we have
    $$\chi^- (d^{\mu^-}_i-d^{\chi^-}_i) \geq  U_i(d^{\mu^-}_i) - U_i(d^{\chi^-}_i)\geq \mu^- (d^{\mu^-}_i-d^{\chi^-}_i).$$
    By multiplying the inequalities above by $-1$, we get the inequality in sub-case (i) and the proof follows directly.
    
  \item [(Case 11: $\sigma_1 \leq b_\mathcal{N}\leq \sigma_2, b_i \leq \sigma_1^i$)] The surplus difference is
  \begin{align*}
   \Delta S_i&=U_i(d^{\pi^+}_i) - \pi^+ ( d^{\pi^+}_i- b_i)- U_i(d^{\mu^+}_i)+ \pi^+ \overline{z}_i.
    \end{align*}
    Since $d^{\pi^+}_i > d^{\mu^+}_i$, we have
    $$\mu^+ (d^{\pi^+}_i-d^{\mu^+}_i) \geq  U_i(d^{\pi^+}_i) - U_i(d^{\mu^+}_i)\geq \pi^+ (d^{\pi^+}_i-d^{\mu^+}_i),$$
    and using the lower bound and $\overline{z}_i=d^{\mu^+}_i-b_i$, we get $\Delta S_i\geq 0$.
  \item [(Case 12: $\sigma_1 \leq b_\mathcal{N}\leq \sigma_2, b_i \geq \sigma_4^i$)] The surplus difference is
  \begin{align*}
   \Delta S_i&=U_i(d^{\pi^+}_i) - \pi^+ ( d^{\pi^+}_i- b_i)- U_i(d^{\mu^-}_i)+ \pi^- \underline{z}_i.
    \end{align*}
    Since $d^{\pi^+}_i < d^{\mu^-}_i$, we have
    $$\pi^+ (d^{\pi^+}_i-d^{\mu^-}_i) \leq  U_i(d^{\pi^+}_i) - U_i(d^{\mu^-}_i)\leq \mu^- (d^{\pi^+}_i-d^{\mu^-}_i),$$
    and using the lower bound and $\underline{z}_i=d^{\mu^-}_i-b_i$, we get $\Delta S_i= (\pi^--\pi^+)\underline{z}_i\geq 0$.
  \item [(Case 13: $\sigma_2 \leq b_\mathcal{N}\leq \sigma_3, b_i \leq \sigma_1^i$)] The surplus difference is
  \begin{align*}
   \Delta S_i&=U_i(d^{\chi^z}_i) - \chi^z ( d^{\chi^z}_i- b_i)- U_i(d^{\mu^+}_i)+ \pi^+ \overline{z}_i.
    \end{align*}
    Since $d^{\chi^z}_i > d^{\mu^+}_i$, we have
    $$\mu^+ (d^{\chi^z}_i-d^{\mu^+}_i) \geq  U_i(d^{\chi^z}_i) - U_i(d^{\mu^+}_i)\geq \chi^z (d^{\chi^z}_i-d^{\mu^+}_i),$$
    and using the lower bound and $\overline{z}_i=d^{\mu^+}_i-b_i$, we get $\Delta S_i= (\pi^+ - \chi^z)\overline{z}_i\geq 0$.
  \item [(Case 14: $\sigma_2 \leq b_\mathcal{N}\leq \sigma_3, b_i \geq \sigma_4^i$)] The surplus difference is
  \begin{align*}
   \Delta S_i&=U_i(d^{\chi^z}_i) - \chi^z ( d^{\chi^z}_i- b_i)- U_i(d^{\mu^-}_i)+ \pi^- \underline{z}_i.
    \end{align*}
    Since $d^{\chi^z}_i < d^{\mu^-}_i$, we have
    $$\chi^z (d^{\chi^z}_i-d^{\mu^-}_i) \leq  U_i(d^{\chi^z}_i) - U_i(d^{\mu^-}_i)\leq \mu^- (d^{\chi^z}_i-d^{\mu^-}_i),$$
    and using the lower bound and $\underline{z}_i=d^{\mu^-}_i-b_i$, we get $\Delta S_i= (\pi^--\chi^z)\underline{z}_i\geq 0$.
   \item [(Case 15: $\sigma_3 \leq b_\mathcal{N}\leq \sigma_4, b_i \leq \sigma_1^i$)] The surplus difference is
  \begin{align*}
   \Delta S_i&=U_i(d^{\pi^-}_i) - \pi^- ( d^{\pi^-}_i- b_i)- U_i(d^{\mu^+}_i)+ \pi^+ \overline{z}_i.
    \end{align*}
    Since $d^{\pi^-}_i > d^{\mu^+}_i$, we have
    $$\mu^+ (d^{\pi^-}_i-d^{\mu^+}_i) \geq  U_i(d^{\pi^-}_i) - U_i(d^{\mu^+}_i)\geq \pi^- (d^{\pi^-}_i-d^{\mu^+}_i),$$
    and using the lower bound and $\overline{z}_i=d^{\mu^+}_i-b_i$, we get $\Delta S_i= (\pi^+-\pi^-)\underline{z}_i\geq 0$.
   \item [(Case 16: $\sigma_3 \leq b_\mathcal{N}\leq \sigma_4, b_i \geq \sigma_4^i$)] The surplus difference is
  \begin{align*}
   \Delta S_i&=U_i(d^{\pi^-}_i) - \pi^- ( d^{\pi^-}_i- b_i)- U_i(d^{\mu^-}_i)+ \pi^- \underline{z}_i.
    \end{align*}
    Since $d^{\pi^-}_i < d^{\mu^-}_i$, we have
    $$\pi^- (d^{\pi^-}_i-d^{\mu^-}_i) \leq  U_i(d^{\pi^-}_i) - U_i(d^{\mu^-}_i)\leq \mu^- (d^{\pi^-}_i-d^{\mu^-}_i),$$
    and using the lower bound and $\underline{z}_i=d^{\mu^-}_i-b_i$, we get $\Delta S_i\geq 0$.
\end{description}
\qed
