# Supplementary material for: Operating-Envelopes-Aware Decentralized Welfare Maximization for Energy Communities
Source: arXiv:2310.07157 source file (2023-10-11)
Supplement: Supplementary file 7 [file MemberLem.tex]

Recall the community member's surplus-maximization problem under the proposed market mechanism. One can easily see that the objective is both concave and differentiable. From KKT conditions, the optimal consumption of every $i\in \mathcal{N}$ community member is:
$$d^{\ast,\chi}_{ik} = \max\{\underline{d}_{ik}, \min\{f_{ik}(\Gamma^\chi(b_\mathcal{N})),\overline{d}_{ik}\}\}, \quad \forall k \in \mathcal{K}.$$
which can be explicitly written as (in vector form)
\begin{equation}\label{eq:OptdiMember}
       \bm{d}^{\ast,\chi}_i = \begin{cases}
           \bm{d}_i^{\chi^+}(b_\mathcal{N}) &,  b_\mathcal{N} \leq \sigma_1\\
          \bm{d}_i^{\pi^+}&,  b_\mathcal{N} \in [\sigma_1,\sigma_2]\\
           \bm{d}_i^{\chi^z}(b_\mathcal{N})&,  b_\mathcal{N} \in [\sigma_2,\sigma_3]\\
            \bm{d}_i^{\pi^-}&,  b_\mathcal{N} \in [\sigma_3,\sigma_4]\\
            \bm{d}_i^{\chi^-}(b_\mathcal{N})&,  b_\mathcal{N} \geq \sigma_4,
       \end{cases}
   \end{equation}
By definition, the optimal net consumption is
\begin{align*}
z^{\ast,\chi}_i &= \bm{1}^\top \bm{d}^{\ast,\chi}_{i} + r_i - g_i=\bm{1}^\top \bm{d}^{\ast,\chi}_{i}-b_i,\nn
\end{align*}
and the aggregate consumption is $ d_\mathcal{N}^\ast = \sum_{i \in \mathcal{N}} \bm{1}^\top \bm{d}^{\ast,\chi}_i$. Lastly, from (\ref{eq:MonotonicPrices1})-(\ref{eq:MonotonicPrices3}), we, respectively, have 
\begin{align*}
    \sum_{i\in \mathcal{N}} \bm{1}^\top \bm{d}_i^{\chi^+}(b_\mathcal{N}) &= b_\mathcal{N}+\overline{z}_\mathcal{N}\nn\\
    \sum_{i\in \mathcal{N}} \bm{1}^\top \bm{d}_i^{\chi^z}(b_\mathcal{N}) &= b_\mathcal{N}\nn\\
    \sum_{i\in \mathcal{N}} \bm{1}^\top \bm{d}_i^{\chi^-}(b_\mathcal{N}) &= b_\mathcal{N}+\underline{z}_\mathcal{N},\nn
\end{align*}
which yields the aggregate net-consumption
\begin{equation*}
       z^{\ast,\chi}_{\mathcal{N}}(b_\mathcal{N}) = d_\mathcal{N}^\ast - b_\mathcal{N} = \begin{cases}
           \overline{z}_\mathcal{N} &,  b_\mathcal{N} \leq \sigma_1\\
          d_\mathcal{N}^\ast - b_\mathcal{N}&,  b_\mathcal{N} \in [\sigma_1,\sigma_2]\\
           0&,  b_\mathcal{N} \in [\sigma_2,\sigma_3]\\
            d_\mathcal{N}^\ast - b_\mathcal{N}&,  b_\mathcal{N} \in [\sigma_3,\sigma_4]\\
            \underline{z}_\mathcal{N}&,  b_\mathcal{N} \geq \sigma_4.
       \end{cases}
   \end{equation*}
\qed
