# Supplementary material for: Operating-Envelopes-Aware Decentralized Welfare Maximization for Energy Communities
Source: arXiv:2310.07157 source file (2023-10-11)
Supplement: Supplementary file 8 [file WelfareLem.tex]

\begin{lemma}[Community maximum welfare]\label{lem:CentralizedWelfare}
   The maximum community welfare under centralized resource scheduling is a monotonically increasing function of $b_\mathcal{N}$ and given by
   \begin{align}
       &W^{\ast,\chi}_\mathcal{N}(b_\mathcal{N}) = \nn\\&\begin{cases}
           \sum_{i\in \mathcal{N}} U_i(\bm{d}_i^{\chi^+}(b_\mathcal{N})) - \pi^+ \overline{z}_\mathcal{N},&\hspace{-.75em} b_\mathcal{N} \leq \sigma_1\\
           \sum_{i\in \mathcal{N}} U_i(\bm{d}_i^{\pi^+}) - \pi^+ (\sum_{i\in \mathcal{N}} \bm{1}^\top \bm{d}_i^{\pi^+}- b_\mathcal{N}),&\hspace{-.75em}  b_\mathcal{N} \in [\sigma_1,\sigma_2]\\
           \sum_{i\in \mathcal{N}} U_i(\bm{d}_i^{\chi^z}(b_\mathcal{N})),&\hspace{-.75em}  b_\mathcal{N} \in [\sigma_2,\sigma_3]\\
            \sum_{i\in \mathcal{N}} U_i(\bm{d}_i^{\pi^-}) - \pi^- (\sum_{i\in \mathcal{N}} \bm{1}^\top \bm{d}_i^{\pi^-}- b_\mathcal{N}),&\hspace{-.75em}  b_\mathcal{N} \in [\sigma_3,\sigma_4]\\
            \sum_{i\in \mathcal{N}} U_i(\bm{d}_i^{\chi^-}(b_\mathcal{N})) - \pi^- \underline{z}_\mathcal{N},&\hspace{-.75em}  b_\mathcal{N} \geq \sigma_4,\label{eq:MaxCentralW}
       \end{cases}
   \end{align}
   where the thresholds $\sigma_1-\sigma_4$ are as computed in the {\em market mechanism} and all consumptions are as defined in (\ref{eq:d+d-}).
\end{lemma}

\subsection*{Proof of Lemma \ref{lem:CentralizedWelfare}}

 Recall the community welfare maximization $\mathcal{P}^\chi_\mathcal{N}$
    \begin{align*}
\begin{array}{lll}\mathcal{P}_{\mathcal{N}}^\chi: &  \underset{\{\bm{d}_i\}_{i=1}^N,\{z_i\}_{i=1}^N}{\rm maximize}& W_\mathcal{N}^\pi := \sum_{i\in \mathcal{N}} S_{i}^{\ast,\chi}(z_i,\bm{b}) \\&\text{subject to} & (\ref{eq:Conslimit})-(\ref{eq:Netconsi}), (\ref{eq:Surplusi}), ~ \forall i\in \mathcal{N}\\&& (\ref{eq:NetconsN})-(\ref{eq:Netconslimit}),(\ref{eq:Pcommunity})-(\ref{eq:ProfitNeutrality}).\end{array}  \end{align*} 
which can be reformulated to the following program, given the profit-neutrality condition:
\begin{align*}
\begin{array}{lll}\underset{\{\bm{d}_i\}_{i=1}^N,\{z_i\}_{i=1}^N}{\rm maximize}& W_\mathcal{N}^\chi:=\sum_{i\in \mathcal{N}} U_i(\bm{d}_i) - P^\pi_\mathcal{N}(z_\mathcal{N}) \\\text{subject to} & 
z_\mathcal{N}=\sum_{i\in \mathcal{N}} z_i= \sum_{i\in \mathcal{N}} (\bm{1}^\top \bm{d}_{i} -b_i) \\&\underline{\bm{d}}_i\preceq \bm{d}_i \preceq \overline{\bm{d}}_i,~~ \forall i\in \mathcal{N}\\& \underline{z}_\mathcal{N} \leq  z_\mathcal{N} \leq \overline{z}_\mathcal{N}, \end{array}   \end{align*} 

Given the problem above, and the assumption in (\ref{eq:ZNfeasibility}), the proof directly follows from Lemma \ref{lem:BenchmarkSur}, as it is a generalization of the benchmark customer problem by adding the dimension of community members. Therefore, the optimal aggregate consumption $d^{\ast,\chi}_\mathcal{N}$ and maximum welfare (objective) $W^{\ast,\chi}_\mathcal{N}$ will be functions of $b_\mathcal{N}:= \sum_{i\in \mathcal{N}} b_i$ rather than $b_i$. The optimal consumption of every member under centralized operation is, therefore,
\begin{equation*}
       \bm{d}^{\ast,\chi}_i(b_\mathcal{N}) = \begin{cases}
           \bm{d}_i^{\chi^+}(b_\mathcal{N}) &,  b_\mathcal{N} \leq \sigma_1\\
          \bm{d}_i^{\pi^+}&,  b_\mathcal{N} \in [\sigma_1,\sigma_2]\\
           \bm{d}_i^{\chi^z}(b_\mathcal{N})&,  b_\mathcal{N} \in [\sigma_2,\sigma_3]\\
            \bm{d}_i^{\pi^-}&,  b_\mathcal{N} \in [\sigma_3,\sigma_4]\\
            \bm{d}_i^{\chi^-}(b_\mathcal{N})&,  b_\mathcal{N} \geq \sigma_4,
       \end{cases}
   \end{equation*}
   which yields the aggregate net-consumption
   \begin{equation*}
       z^{\ast,\chi}_{\mathcal{N}}(b_\mathcal{N}) = \begin{cases}
           \overline{z}_\mathcal{N} &,  b_\mathcal{N} \leq \sigma_1\\
          \bm{1}^\top \bm{d}_i^{\pi^+} - b_\mathcal{N}&,  b_\mathcal{N} \in [\sigma_1,\sigma_2]\\
           0&,  b_\mathcal{N} \in [\sigma_2,\sigma_3]\\
            \bm{1}^\top \bm{d}_i^{\pi^-} - b_\mathcal{N}&,  b_\mathcal{N} \in [\sigma_3,\sigma_4]\\
            \underline{z}_\mathcal{N}&,  b_\mathcal{N} \geq \sigma_4.
       \end{cases}
   \end{equation*}
The maximum welfare can be directly computed plugging $d^{\ast,\chi}_\mathcal{N}(b_\mathcal{N})$ and $z^{\ast,\chi}_{\mathcal{N}}(b_\mathcal{N})$ into $W^{\ast,\chi}_\mathcal{N}= \sum_{i\in \mathcal{N}} U_i(\bm{d}^{\ast,\chi}_i(b_\mathcal{N})) - P^{\ast,\pi}_\mathcal{N}(z^{\ast,\chi}_{\mathcal{N}}(b_\mathcal{N}))$, which gives (\ref{eq:MaxCentralW}). \qed
